# Supplementary material for: Bayesian Multinomial Logistic Normal Additive Regression for Microbiome Data Analysis
Source: arXiv:2410.03911 source file (2026-11-10)
Supplement: Supplementary file 2 [file Supplement.tex]

\documentclass[
  12pt]{article}

\usepackage{amsthm}
\usepackage{amsfonts}
\usepackage{graphicx,psfrag,epsf}
\usepackage{enumerate}
\usepackage{natbib}
\usepackage{algorithm}
\usepackage{algpseudocode}
\usepackage{fix-cm}
\usepackage{makecell} % Allows multi-line text in table cells
\usepackage{pifont}
\usepackage{caption}
\usepackage[colorlinks,citecolor=blue,urlcolor=blue,linkcolor = purple]{hyperref}%% uncomment this for coloring bibliography citations and linked URLs

\usepackage{amsmath,amssymb}
\usepackage{iftex}
\ifPDFTeX
  \usepackage[T1]{fontenc}
  \usepackage[utf8]{inputenc}
  \usepackage{textcomp} % provide euro and other symbols
\else % if luatex or xetex
  \usepackage{unicode-math}
  \defaultfontfeatures{Scale=MatchLowercase}
  \defaultfontfeatures[\rmfamily]{Ligatures=TeX,Scale=1}
\fi
\usepackage{lmodern}
\ifPDFTeX\else  
    % xetex/luatex font selection
\fi
% Use upquote if available, for straight quotes in verbatim environments
\IfFileExists{upquote.sty}{\usepackage{upquote}}{}
\IfFileExists{microtype.sty}{% use microtype if available
  \usepackage[]{microtype}
  \UseMicrotypeSet[protrusion]{basicmath} % disable protrusion for tt fonts
}{}
\makeatletter
\@ifundefined{KOMAClassName}{% if non-KOMA class
  \IfFileExists{parskip.sty}{%
    \usepackage{parskip}
  }{% else
    \setlength{\parindent}{0pt}
    \setlength{\parskip}{6pt plus 2pt minus 1pt}}
}{% if KOMA class
  \KOMAoptions{parskip=half}}
\makeatother
\usepackage{xcolor}
\setlength{\emergencystretch}{3em} % prevent overfull lines
\setcounter{secnumdepth}{5}
% Make \paragraph and \subparagraph free-standing
\makeatletter
\ifx\paragraph\undefined\else
  \let\oldparagraph\paragraph
  \renewcommand{\paragraph}{
    \@ifstar
      \xxxParagraphStar
      \xxxParagraphNoStar
  }
  \newcommand{\xxxParagraphStar}[1]{\oldparagraph*{#1}\mbox{}}
  \newcommand{\xxxParagraphNoStar}[1]{\oldparagraph{#1}\mbox{}}
\fi
\ifx\subparagraph\undefined\else
  \let\oldsubparagraph\subparagraph
  \renewcommand{\subparagraph}{
    \@ifstar
      \xxxSubParagraphStar
      \xxxSubParagraphNoStar
  }
  \newcommand{\xxxSubParagraphStar}[1]{\oldsubparagraph*{#1}\mbox{}}
  \newcommand{\xxxSubParagraphNoStar}[1]{\oldsubparagraph{#1}\mbox{}}
\fi
\makeatother

\usepackage{longtable,booktabs,array}
\usepackage{calc} % for calculating minipage widths
% Correct order of tables after \paragraph or \subparagraph
\usepackage{etoolbox}
\makeatletter
\patchcmd\longtable{\par}{\if@noskipsec\mbox{}\fi\par}{}{}
\makeatother
% Allow footnotes in longtable head/foot
\IfFileExists{footnotehyper.sty}{\usepackage{footnotehyper}}{\usepackage{footnote}}
\makesavenoteenv{longtable}
\usepackage{graphicx}
\makeatletter
\def\maxwidth{\ifdim\Gin@nat@width>\linewidth\linewidth\else\Gin@nat@width\fi}
\def\maxheight{\ifdim\Gin@nat@height>\textheight\textheight\else\Gin@nat@height\fi}
\makeatother
% Scale images if necessary, so that they will not overflow the page
% margins by default, and it is still possible to overwrite the defaults
% using explicit options in \includegraphics[width, height, ...]{}
\setkeys{Gin}{width=\maxwidth,height=\maxheight,keepaspectratio}
% Set default figure placement to htbp
\makeatletter
\def\fps@figure{htbp}
\makeatother

\addtolength{\oddsidemargin}{-.5in}%
\addtolength{\evensidemargin}{-.1in}%
\addtolength{\textwidth}{1in}%
\addtolength{\textheight}{1.7in}%
\addtolength{\topmargin}{-1in}
\makeatletter
\@ifpackageloaded{caption}{}{\usepackage{caption}}
\AtBeginDocument{%
\ifdefined\contentsname
  \renewcommand*\contentsname{Table of contents}
\else
  \newcommand\contentsname{Table of contents}
\fi
\ifdefined\listfigurename
  \renewcommand*\listfigurename{List of Figures}
\else
  \newcommand\listfigurename{List of Figures}
\fi
\ifdefined\listtablename
  \renewcommand*\listtablename{List of Tables}
\else
  \newcommand\listtablename{List of Tables}
\fi
\ifdefined\figurename
  \renewcommand*\figurename{Figure}
\else
  \newcommand\figurename{Figure}
\fi
\ifdefined\tablename
  \renewcommand*\tablename{Table}
\else
  \newcommand\tablename{Table}
\fi
}
\@ifpackageloaded{float}{}{\usepackage{float}}
\floatstyle{ruled}
\@ifundefined{c@chapter}{\newfloat{codelisting}{h}{lop}}{\newfloat{codelisting}{h}{lop}[chapter]}
\floatname{codelisting}{Listing}

\makeatother
\makeatletter
\makeatother
\makeatletter
\@ifpackageloaded{caption}{}{\usepackage{caption}}
\@ifpackageloaded{subcaption}{}{\usepackage{subcaption}}
\makeatother

\ifLuaTeX
  \usepackage{selnolig}  % disable illegal ligatures
\fi
\usepackage[]{natbib}
\bibliographystyle{agsm}
\usepackage{bookmark}

\IfFileExists{xurl.sty}{\usepackage{xurl}}{} % add URL line breaks if available
\urlstyle{same} % disable monospaced font for URLs
\hypersetup{
  pdftitle={Title},
  pdfauthor={Author 1; Author 2},
  pdfkeywords={3 to 6 keywords, that do not appear in the title},
  colorlinks=true,
  linkcolor={purple},
  filecolor={Maroon},
  citecolor={blue},
  urlcolor={purple},
  pdfcreator={LaTeX via pandoc}}

\newcommand{\anon}{1}

% \startlocaldefs

%%%%%%%%%%%%%%%%%%%%%%%%%%%%%%%%%%%%%%%%%%%%%%
%%                                          %%
%% For Axiom, Claim, Corollary, Hypothesis, %%
%% Lemma, Theorem, Proposition              %%
%% use \theoremstyle{plain}                 %%
%%                                          %%
%%%%%%%%%%%%%%%%%%%%%%%%%%%%%%%%%%%%%%%%%%%%%%
\theoremstyle{plain}

\newtheorem{theorem}{Theorem}[section]

%%%%%%%%%%%%%%%%%%%%%%%%%%%%%%%%%%%%%%%%%%%%%%
%%                                          %%
%% For Assumption, Definition, Example,     %%
%% Notation, Property, Remark, Fact         %%
%% use \theoremstyle{remark}                %%
%%                                          %%
%%%%%%%%%%%%%%%%%%%%%%%%%%%%%%%%%%%%%%%%%%%%%%
\theoremstyle{remark}

%%%%%%%%%%%%%%%%%%%%%%%%%%%%%%%%%%%%%%%%%%%%%%
%% Please put your definitions here:        %%
%%%%%%%%%%%%%%%%%%%%%%%%%%%%%%%%%%%%%%%%%%%%%%

  % Infimum, note: * undersets limits
  % Infimum, note: * undersets limits

 % Real Space
 % Simplex
 % Integers

% \endlocaldefs

\pdfminorversion=4

\begin{document}

\def\spacingset#1{\renewcommand{\baselinestretch}%
{#1}\small\normalsize} \spacingset{1}

%%%%%%%%%%%%%%%%%%%%%%%%%%%%%%%%%%%%%%%%%%%%%%%%%%%%%%%%%%%%%%%%%%%%%%%%%%%%%%

\if1\anon
{
  \title{\bf Supplement Materials of Scalable Bayesian Semiparametric
Additive Regression Models For Microbiome Studies}
  \author{Tinghua Chen\\
    College of Information Science and Technology, \\
    Pennsylvania State University\\
    and \\
     Michelle Pistner Nixon \\
    College of Information Science and Technology, \\
    Pennsylvania State University\\
    and \\
    Justin D. Silverman\\
    College of Information Science and Technology, \\
    Department of Statistics,\\
    Department of Medicine,\\
    Pennsylvania State University}
  \maketitle
} \fi

\if0\anon
{
  \bigskip
  \bigskip

  \bigskip
  \begin{center}
    {\LARGE\bf Title}
\end{center}
  \medskip
} \fi

\spacingset{1.8} % DON'T change the spacing!

\section{Review of the Collapsed-Uncollapsed (CU) Sampler}
\label{sec:Marginally LTP}

% \subsection{Collapsed-Uncollapsed (CU) Sampler}
% \label{sec:cu-sampler}
The definition of MLTPs is key to efficient inference. If a model \(p(\mathbf{Y}, \mathbf{H}, \mathbf{\Phi})\) has a closed-form marginal \(p(\mathbf{Y}, \mathbf{H})\) that is an LTP, then its closed form conditional \(p(\mathbf{\Phi} \mid \mathbf{Y}, \mathbf{H})\) likely exists. We call the marginal \(p(\mathbf{Y}, \mathbf{H})\) the \textit{collapsed form} and \(p(\mathbf{\Phi} \mid \mathbf{Y}, \mathbf{H})\) the \textit{uncollapsed form}. The posterior of an MLTP factors as
\[p(\mathbf{H},\mathbf{\Phi} \mid \mathbf{Y})=p(\mathbf{\Phi}\mid \mathbf{H}, \mathbf{Y})p(\mathbf{H} \mid \mathbf{Y})\]
with the uncollapsed form as the first term and the posterior of the collapsed form as the second. 
As the collapsed form is rarely conjugate, techniques such as MCMC can be used to obtain samples from it's posterior. Then, conditioned on those samples, the uncollapsed form can be used to obtain samples from the joint posterior. Especially when \(\boldsymbol{\Phi}\) is high-dimensional, this \textit{Collapse-Uncollapse} sampler can be much more efficient than common alternatives~\citep{silverman2022bayesian}. Still, the most substantial enhancements occur when approximations to the collapsed form are considered. 

We have developed a Laplace approximation for the collapsed form of MLTPs:
\[p(\text{vec}(\mathbf{H})\mid \mathbf{Y})\approx \mathcal{N}(\text{vec}(\hat{\mathbf{H}}),\nabla^{-2}[\text{vec}(\hat{\mathbf{H}})])\]
where \(\hat{\mathbf{H}}\) denotes the \textit{Maximum A Posteriori (MAP)} estimate of the collapsed form and \(\nabla^{-2}[\text{vec}(\hat{\mathbf{H}})]\) denotes the inverse Hessian of the collapsed form evaluated at the MAP estimate. The derived analytical results for the gradient and Hessian of the collapsed form is in Supplement section \ref{sec:LA}. 
Focusing on applications to MultiAddGPs, we proved error bounds on the Laplace approximation and provided simulation and real analyses showing that the approximation was extremely accurate in the context of microbiome data analysis. 
Beyond the accuracy of posterior calculations, we showed that this CU sampler with the Laplace approximation (simply referred to as the CU sampler in the following text) was often 4-5 orders of magnitude faster than MCMC and 1-2 orders of magnitude faster than black-box variational inference while also being more accurate than the later.

\section{MultiAddGPs as Marginal Latent Matrix-t Process (MLTPs)}
\label{sec:proof}
\subsection{Derivation of Collapsed form}

\begin{theorem}
  MultiAddGPs are MLTPs with parameters  $\boldsymbol{\Phi} = \{\mathbf{F},\mathbf{B}, \mathbf{f}^{(1)}, \dots, \mathbf{f}^{(K)}, \boldsymbol{\Sigma}\}$. The collapsed form \(p( \mathbf{Y},\mathbf{H})\) is an LTP:
  \begin{align*}
  \mathbf{Y}_{\cdot n} &\sim \text{Multinomial}(\mathbf{\Pi}_{\cdot n}) \\ 
    \mathbf{\Pi}_{\cdot n} &= \phi^{-1}(\mathbf{H}_{\cdot n}) \\
    \mathbf{H} &\sim TP(\nu, \mathbf{M}, \mathbf{V}, \mathbf{A})
  \end{align*}
 where $\phi$ is an invertible log-ratio transformation, $  \mathbf{M}=\boldsymbol{\Theta}^{(0)}\mathbf{X} + \sum_{k=1}^K\boldsymbol{\Theta}^{(k)}(\mathbf{Z}^{(k)})$, $\mathbf{V} = \boldsymbol{\Xi}$, and $\mathbf{A} = \mathbf{X}^{T} \boldsymbol{\Gamma}^{(0)} \mathbf{X} + \sum_{k=1}^{K} \boldsymbol{\Gamma}^{(k)}(\mathbf{Z}^{(k)}) + \mathbf{I}_N, \nu =\zeta  $
 \end{theorem}
\begin{proof}
    We prove this theorem by showing that the marginal of MultiAddGP models is an LTP. By definition 2 from~\citep{silverman2022bayesian}, if $p(\mathbf{H,Y})$ is an LTP, then $p(\mathbf{H,Y,F},\mathbf{f}^{(1)},\dots,\mathbf{f}^{(K)},\mathbf{\Sigma})$ is a MLTP model.  To begin with, we note that Equation (4) in the main text (along with its priors) can alternatively be written as:
    \begin{align}
        \mathbf{H} &= \mathbf{F}+\mathbf{E}^{\mathbf{H}} \hspace{1.2cm} \mathbf{E}^{\mathbf{H}} \sim N(0,\boldsymbol{\Sigma},\mathbf{I}_N) \label{eq:H}\\
        \mathbf{F} &= \mathbf{BX} + \sum_{k=1}^{K} \mathbf{f}^{(k)}(\mathbf{Z}^{(k)}) \label{eq:F}\\
        \mathbf{B} &= \boldsymbol{\Theta}^{(0)} + \mathbf{E}^{\mathbf{B}} \hspace{0.8cm} \mathbf{E}^{\mathbf{B}} \sim N(0,\mathbf{\Sigma,\Gamma}^{(0)}) \label{eq:B}\\
        \mathbf{f}^{(k)} &= \boldsymbol{\Theta}^{(k)} +  \mathbf{E}^{\mathbf{f}^{(k)}} \hspace{0.3cm} \mathbf{E}^{\mathbf{f}^{(k)}} \sim N(0,\mathbf{\Sigma,\Gamma}^{(k)}) \label{eq:f}\\
        \boldsymbol{\Sigma} &\sim IW(\mathbf{\Xi}, \zeta) \label{eq:Sigma}
    \end{align}
    Using this form in combination with the affine transformation property of the matrix normal distribution, it is straightforward to marginalize over $\mathbf{B}$ and $\mathbf{f}^{(k)}$ producing the following form:
    \begin{align}
        \mathbf{F} &=\boldsymbol{\Theta}^{(0)}\mathbf{X} + \sum_{k=1}^{K}\boldsymbol{\Theta}^{(k)}(\mathbf{Z}^{(k)}) +\mathbf{E}^{\mathbf{B}} + \mathbf{E}^{\mathbf{f}^{(k)}}  \hspace{0.2cm} \mathbf{E}^{\mathbf{B}} \sim N(0,\boldsymbol{\Sigma},\boldsymbol{\Gamma}^{(0)})  \hspace{0.2cm} \mathbf{E}^{\mathbf{f}^{(k)}} \sim N(0,\boldsymbol{\Sigma},\boldsymbol{\Gamma}^{(k)})     \label{eq:Marginalize_B_f_1}\\
        \mathbf{F} &= \boldsymbol{\Theta}^{(0)}\mathbf{X} + \sum_{k=1}^{K}\boldsymbol{\Theta}^{(k)}(\mathbf{Z}^{(k)}) + \mathbf{E}^{\mathbf{F}}  \hspace{0.2cm} \mathbf{E}^{\mathbf{F}} \sim N(0, \boldsymbol{\Sigma},\mathbf{X}^T\boldsymbol{\Gamma}^{(0)}\mathbf{X}+\sum_{k=1}^{K}\boldsymbol{\Gamma}^{(k)}(\mathbf{Z}^{(k)}))  \label{eq:Marginalize_B_f_2}
    \end{align}
    Thus we may rewrite Equations (\ref{eq:H}) - (\ref{eq:Sigma}) as
    \begin{align}
        \mathbf{H} &= \mathbf{F}+\mathbf{E}^{\mathbf{H}} \hspace{1.2cm} \mathbf{E}^{\mathbf{H}} \sim N(0,\boldsymbol{\Sigma},\mathbf{I}_N) \label{eq:H2}\\
       \mathbf{F} &= \boldsymbol{\Theta}^{(0)}\mathbf{X} + \sum_{k=1}^{K}\boldsymbol{\Theta}^{(k)}(\mathbf{Z}^{(k)}) + \mathbf{E}^{\mathbf{F}}  \hspace{0.2cm} \mathbf{E}^{\mathbf{F}} \sim N(0, \boldsymbol{\Sigma},\mathbf{X}^T\boldsymbol{\Gamma}^{(0)}\mathbf{X}+\sum_{k=1}^{K}\boldsymbol{\Gamma}^{(k)}(\mathbf{Z}^{(k)}))   \label{eq:F2} \\
        \boldsymbol{\Sigma} &\sim IW(\boldsymbol{\Xi}, \zeta) \label{eq:Sigma2}
    \end{align}
    Following the result from \cite{gupta2018matrix}, we can marginalize over $\mathbf{F}$ and $\boldsymbol{\Sigma}$ in Equations (\ref{eq:F2}) and (\ref{eq:Sigma2}) to get 
    \begin{align*}
        \mathbf{H} \sim TP(\zeta,\boldsymbol{\Theta}^{(0)}\mathbf{X} + \sum_{k=1}^{K}\boldsymbol{\Theta}^{(k)}(\mathbf{Z}^{(k)}) ,\mathbf{\Xi},\mathbf{X}^T\boldsymbol{\Gamma}^{(0)}\mathbf{X}+\sum_{k=1}^{K}\boldsymbol{\Gamma}^{(k)}(\mathbf{Z}^{(k)}) + \mathbf{I}_N)
    \end{align*}
    Finally, incorporating Equations (2) and (3) allows us to write the marginalized form of the MultiAddGP model as an LTP
    \begin{align*}
          \boldsymbol{Y} &\sim g(\boldsymbol{\Pi}, \lambda) \\
          \boldsymbol{\Pi}&=\phi^{-1}(\boldsymbol{H}) \\
          \boldsymbol{H} &\sim TP(\nu, \boldsymbol{M}, \boldsymbol{V}, \boldsymbol{A}). 
    \end{align*}
    where $g$ is product multinomial, $\phi$ is an invertible log-ratio transformation, $  \mathbf{M}=\boldsymbol{\Theta}^{(0)}\mathbf{X} + \sum_{k=1}^K\boldsymbol{\Theta}^{(k)}(\mathbf{Z}^{(k)})$, $\mathbf{V} = \boldsymbol{\Xi}$, and $\mathbf{A} = \mathbf{X}^{T} \boldsymbol{\Gamma}^{(0)} \mathbf{X} + \sum_{k=1}^{K} \boldsymbol{\Gamma}^{(k)}(\mathbf{Z}^{(k)}) + \mathbf{I}_N, \nu =\zeta  $
\end{proof}

\subsection{Derivation of Uncollapsed form - Sample from $p(\mathbf{F}, \boldsymbol{\Sigma}|\mathbf{H}, \mathbf{Y})$}

Here, we demonstrate how to efficiently compute and sample from the conditional posterior \( p(\mathbf{F}, \boldsymbol{\Sigma}|\mathbf{H}, \mathbf{Y}, \mathbf{X}, \mathbf{Z}) \). Since \(\mathbf{F}\) and \(\boldsymbol{\Sigma}\) are conditionally independent of \(\mathbf{Y}\) given \(\mathbf{H}\), by applying the chain rule, we can rewrite the equation as:
\begin{align}
p(\mathbf{F},\boldsymbol{\Sigma}|\mathbf{H}, \mathbf{Y}, \mathbf{X}, \mathbf{Z}) &=
p(\mathbf{F}|\boldsymbol{\Sigma},\mathbf{H},\mathbf{X},\mathbf{Z})p(\boldsymbol{\Sigma}|\mathbf{H},\mathbf{X},\mathbf{Z}) \nonumber
\end{align}
To proceed, we clarify the notation used to distinguish between \emph{smoothing} and \emph{prediction}. Smoothing refers to inferring latent quantities over observed covariates $(\mathbf{X}^o, \mathbf{Z}^o)$, while prediction refers to inferring latent quantities over unobserved covariates $(\mathbf{X}^u, \mathbf{Z}^u)$. We thus define the expanded notation:
\begin{align*}
    \mathbf{X} &= \begin{bmatrix} \mathbf{X}^o & \mathbf{X}^u \end{bmatrix}, \quad
    \mathbf{Z} = \begin{bmatrix} \mathbf{Z}^o & \mathbf{Z}^u \end{bmatrix}, \\
    \boldsymbol{\Sigma} &= \begin{bmatrix} 
    \boldsymbol{\Sigma}^{oo} & (\boldsymbol{\Sigma}^{uo})^T \\
    \boldsymbol{\Sigma}^{uo} & \boldsymbol{\Sigma}^{uu} 
    \end{bmatrix}, \quad
    \mathbf{F} = \begin{bmatrix} \mathbf{F}^o & \mathbf{F}^u \end{bmatrix}, \\
    \boldsymbol{\Theta} &= \begin{bmatrix} \boldsymbol{\Theta}^o & \boldsymbol{\Theta}^u \end{bmatrix}, \quad
    \boldsymbol{\Gamma} = \begin{bmatrix} 
    \boldsymbol{\Gamma}^{oo} & (\boldsymbol{\Gamma}^{uo})^T \\
    \boldsymbol{\Gamma}^{uo} & \boldsymbol{\Gamma}^{uu} 
    \end{bmatrix}.
\end{align*}
where
\begin{align*}
    \boldsymbol{\Theta}^o &= \boldsymbol{\Theta}^{(0)} \mathbf{X}^{o} - \sum_{k=1}^K \boldsymbol{\Theta}^{(k)}(\mathbf{Z}^{(k),o}), \\
    \boldsymbol{\Theta}^u &= \boldsymbol{\Theta}^{(0)} \mathbf{X}^{u} - \sum_{k=1}^K \boldsymbol{\Theta}^{(k)}(\mathbf{Z}^{(k),u}), \\
    \boldsymbol{\Gamma}^{oo} &= \mathbf{X}^{T,o} \boldsymbol{\Gamma}^{(0)} \mathbf{X}^{o} + \sum_{k=1}^K \boldsymbol{\Gamma}^{(k)}(\mathbf{Z}^{(k),o}), \\
    \boldsymbol{\Gamma}^{uu} &= \mathbf{X}^{T,u} \boldsymbol{\Gamma}^{(0)} \mathbf{X}^{u} + \sum_{k=1}^K \boldsymbol{\Gamma}^{(k)}(\mathbf{Z}^{(k),u}), \\
    \boldsymbol{\Gamma}^{uo} &= \mathbf{X}^{T} \boldsymbol{\Gamma}^{(0)} \mathbf{X} + \sum_{k=1}^K \boldsymbol{\Gamma}^{(k)}(\mathbf{Z}^{(k),o}, \mathbf{Z}^{(k),u}).
\end{align*}
Let $D = D_o + D_u$ and $N = N_o + N_u$ denote the total dimensionality of $\boldsymbol{\Sigma}$ and $\boldsymbol{\Gamma}$.
To sample from $p(\mathbf{F} \mid \boldsymbol{\Sigma}, \mathbf{H}, \mathbf{X}, \mathbf{Z})$ and $p(\boldsymbol{\Sigma} \mid \mathbf{H}, \mathbf{X}, \mathbf{Z})$, we define:$\boldsymbol{\Sigma}^{ou/oo} = (\boldsymbol{\Sigma}^{oo})^{-1} (\boldsymbol{\Sigma}^{uo})^T $ and $
\boldsymbol{\Sigma}^{uu \cdot oo} = \boldsymbol{\Sigma}^{uu} - \boldsymbol{\Sigma}^{uo} \boldsymbol{\Sigma}^{ou/oo}.
$ and using the conditional properties of the inverse-Wishart distribution~\cite{gupta2018matrix}, we sample $\boldsymbol{\Sigma}$ and $\mathbf{F}$ from following:
\begin{align*}
\boldsymbol{\Sigma}^{uu \cdot oo} &\sim \mathcal{IW}(\boldsymbol{\Xi}^{uu \cdot oo}, \zeta + D), \\
\boldsymbol{\Sigma}^{ou/oo} \mid \boldsymbol{\Sigma}^{uu \cdot oo} &\sim \mathcal{N}(\boldsymbol{\Xi}^{ou/oo}, (\boldsymbol{\Xi}^{oo})^{-1}, \boldsymbol{\Sigma}^{uu \cdot oo}), \\
\boldsymbol{\Sigma} &= \begin{bmatrix}
(\boldsymbol{\Sigma}^{oo})^{-1} + \boldsymbol{\Sigma}^{ou/oo} (\boldsymbol{\Sigma}^{uu \cdot oo})^{-1} (\boldsymbol{\Sigma}^{ou/oo})^T & -\boldsymbol{\Sigma}^{ou/oo} (\boldsymbol{\Sigma}^{uu \cdot oo})^{-1} \\
-(\boldsymbol{\Sigma}^{uu \cdot oo})^{-1} (\boldsymbol{\Sigma}^{ou/oo})^T & (\boldsymbol{\Sigma}^{uu \cdot oo})^{-1}\end{bmatrix}.\\
\mathbf{F}^u \mid \mathbf{F}^o, \boldsymbol{\Sigma} &\sim \mathcal{N}\left( \boldsymbol{\Theta}^u + (\mathbf{F}^o - \boldsymbol{\Theta}^o)\boldsymbol{\Gamma}^{ou/oo}, \boldsymbol{\Sigma}, \boldsymbol{\Gamma}^{uu} - \boldsymbol{\Gamma}^{uo} (\boldsymbol{\Gamma}^{oo})^{-1} \boldsymbol{\Gamma}^{ou} \right).
\end{align*}

\section{Laplace Approximation in the Collapsed Step}
\label{sec:LA}
The Laplace approximation for the collapsed step involves three main steps: 
(1) obtaining the MAP estimate $\mathbf{\hat{H}}$ via optimization, 
(2) computing the Hessian matrix $\nabla^{-2}\text{vec}(\hat{\mathbf{H}})$ at the MAP estimate, 
and (3) sampling from the approximating Gaussian distribution $\mathcal{N}(\text{vec}(\hat{\mathbf{H})}, \nabla^{-2}(\text{vec}\hat{\mathbf{H}}))$.
The MAP estimate of $\mathbf{H}$ is obtained by solving the following optimization problem:
\begin{align*}
    \hat{\mathbf{H}} & = \arg\min_{\mathbf{H}} \left\{ \log p(\mathbf{H} \mid \mathbf{Y}) \right\} \\
    & \propto \arg\min_{\mathbf{H}} \left\{ -\log g(\mathbf{Y} \mid \phi^{-1}(\mathbf{H})) - \log p(\mathbf{H}) \right\}.
\end{align*}
We use the L-BFGS optimizer to solve this problem, which requires computing the gradient of the negative log-posterior:
\[
- \frac{d \log p(\mathbf{H} \mid \mathbf{Y})}{d \mathbf{\text{vec}(H)}} 
= - \frac{d \log g(\mathbf{Y} \mid \phi^{-1}(\mathbf{H}))}{d \mathbf{\text{vec}(H)}} 
- \frac{d \log p(\mathbf{H})}{d \mathbf{\text{vec}(H)}}.
\]
The two gradient components are computed as follows:
\begin{align}
    -\frac{d \log g(\mathbf{Y} \mid \phi^{-1}(\mathbf{H}))}{d \mathbf{\text{vec}(H)}} 
    &= \left( \text{vec}(\mathbf{Y}) - \text{vec}(I_D I_D^T \mathbf{Y}) \odot J \right)^T,
    \label{eq:gradient_Y}
\end{align}
\begin{align}
    -\frac{d \log p(\mathbf{H})}{d \mathbf{\text{vec}(H)}} 
    &= \text{vec} \left( (\mathbf{R} + \mathbf{R}^T)\mathbf{C}^T \right)^T,
    \label{eq:gradient_H}
\end{align}
where:
\begin{align*}
    J &= \text{vec} \left( \exp(\mathbf{H}) \right) \oslash 
    \text{vec} \left( I_{D-1} (I + \exp(\mathbf{H})^T I_{D-1})^T \right), \\
    \mathbf{R} &= \left( I_P + \mathbf{V}^{-1} (\mathbf{H} - \mathbf{M}) \mathbf{A}^{-1} (\mathbf{H} - \mathbf{M})^T \right)^{-1} \mathbf{V}^{-1}, \\
    \mathbf{C} &= \mathbf{A}^{-1} (\mathbf{H}^T - \mathbf{M}^T).
\end{align*}
Once the MAP estimate $\hat{\mathbf{H}}$ has been obtained, we compute the Hessian at that point:
\[
\nabla^{-2}[\hat{\mathbf{H}}] = \nabla^{-2} \log g(\mathbf{Y} \mid \phi^{-1}(\hat{\mathbf{H}})) + \nabla^{-2} \log p(\hat{\mathbf{H}}).
\]
Using equations \eqref{eq:gradient_Y} and \eqref{eq:gradient_H}, the Hessians of the likelihood and prior terms are given by:
\begin{align*}
    \nabla^{-2} \log g(\mathbf{Y} \mid \phi^{-1}(\mathbf{H})) &= \text{diag}(W^{(1)}, \dots, W^{(N)}), \\
    \nabla^{-2} \log p(\mathbf{H}) &= \left( A^{-1} \otimes (R + R^T) \right) - (L + L^T) \\
    &\quad - T_{N,D-1} \left[ (RC^T \otimes CR^T) + (R^T C^T \otimes CR) \right],
\end{align*}
where:
\begin{align*}
    W^{(j)} &= I_D^T Y \left( J_{(j)} J_{(j)}^T - \text{diag}(J_{(j)}) \right), \\
    L &= \mathbf{C} \mathbf{R} \mathbf{C}^T \otimes \mathbf{R}^T,
\end{align*}

\noindent and \( T_{N,D-1} \) is an \( N(D-1) \times N(D-1) \) permutation matrix.
Finally, we draw samples from the approximating Gaussian distribution. The Laplace approximation to the posterior \( p(\mathbf{H} \mid \mathbf{Y}) \) is given by:
\[
q(\mathbf{H} \mid \mathbf{Y}) =\mathcal{N}(\text{vec}(\hat{\mathbf{H})}, \nabla^{-2}(\text{vec}\hat{\mathbf{H}})).
\]
In practice, to avoid explicit matrix inversion when sampling, we apply the Cholesky decomposition of the Hessian.

\section{Derivation of the posterior distribution of Matrix Normal}
\label{sec:matrix_normal}
\begin{theorem} 
If
\begin{align*}
\mathbf{Y} \mid \mathbf{\Lambda} &\sim \mathcal{MN}(\mathbf{\Lambda X}, \mathbf{\Sigma}, \mathbf{\Gamma})\\
\mathbf{\Lambda} &\sim \mathcal{MN}(\mathbf{\Theta}, \mathbf{\Sigma}, \mathbf{Z}) 
\end{align*}
and \(\mathbf{\Sigma}\) is known, then the posterior of \(\mathbf{\Lambda}\) is given by:
\[\mathbf{\Lambda} \mid \mathbf{\Sigma}, \mathbf{Y} \sim \mathcal{MN}\left( (\mathbf{Y} \mathbf{\Gamma}^{-1} \mathbf{X}^T + \mathbf{\Theta} \mathbf{Z}^{-1}) (\mathbf{X} \mathbf{\Gamma}^{-1} \mathbf{X}^T + \mathbf{Z}^{-1})^{-1}, \mathbf{\Sigma}, (\mathbf{X} \mathbf{\Gamma}^{-1} \mathbf{X}^T + \mathbf{Z}^{-1})^{-1} \right) \]
\end{theorem}
\begin{proof}
Using the density function of the matrix normal distribution, we can write:
\[
\mathbf{\Lambda} \mid \mathbf{Y} \propto \exp\left[ -\frac{1}{2} \text{tr} \left( \mathbf{\Sigma}^{-1} (\mathbf{Y} - \mathbf{\Lambda} \mathbf{X}) \mathbf{\Gamma}^{-1} (\mathbf{Y} - \mathbf{\Lambda} \mathbf{X})^T \right) \right] \times \exp\left[ -\frac{1}{2} \text{tr} \left( \mathbf{\Sigma}^{-1} (\mathbf{\Lambda} - \mathbf{\Theta}) \mathbf{Z}^{-1} (\mathbf{\Lambda} - \mathbf{\Theta})^T \right) \right]
\]
Combining the exponents and expanding the term:
\begin{align*}
&\propto \exp\left[ -\frac{1}{2} \operatorname{tr}  \left(\mathbf{\Sigma}^{-1} \left( \mathbf{Y} \mathbf{\Gamma}^{-1} \mathbf{Y}^T - \mathbf{\Lambda} \mathbf{X} \mathbf{\Gamma}^{-1} \mathbf{Y}^T - \mathbf{Y} \mathbf{\Gamma}^{-1} \mathbf{X}^T \mathbf{\Lambda}^T + \mathbf{\Lambda} \mathbf{X} \mathbf{\Gamma}^{-1} \mathbf{X}^T \mathbf{\Lambda}^T \right. \right. \right. \\
&\quad \left. \left. \left. + \mathbf{\Lambda} \mathbf{Z}^{-1} \mathbf{\Lambda}^T - \mathbf{\Theta} \mathbf{Z}^{-1} \mathbf{\Lambda}^T - \mathbf{\Lambda} \mathbf{Z}^{-1} \mathbf{\Theta}^T + \mathbf{\Theta} \mathbf{Z}^{-1} \mathbf{\Theta}^T \right) \right) \right].
\end{align*}
\begin{align*}
& \propto \exp\left[ -\frac{1}{2} \text{tr} \left( \mathbf{\Sigma}^{-1} \left( -\mathbf{\Lambda} \mathbf{X} \mathbf{\Gamma}^{-1} \mathbf{Y}^T - \mathbf{Y} \mathbf{\Gamma}^{-1} \mathbf{X}^T \mathbf{\Lambda}^T + \mathbf{\Lambda} \mathbf{X} \mathbf{\Gamma}^{-1} \mathbf{X}^T \mathbf{\Lambda}^T + \mathbf{\Lambda} \mathbf{Z}^{-1} \mathbf{\Lambda}^T \right. \right. \right. \\
&\quad \left. \left. \left. -\mathbf{\Theta} \mathbf{Z}^{-1} \mathbf{\Lambda}^T - \mathbf{\Lambda} \mathbf{Z}^{-1} \mathbf{\Theta}^T \right) \right) \right]
\end{align*}
Grouping like terms:
\[
\mathbf{\Lambda} \mid \mathbf{Y} \propto \exp\left[ -\frac{1}{2} \text{tr} \left( \mathbf{\Sigma}^{-1} \left( \mathbf{\Lambda} (\mathbf{X} \mathbf{\Gamma}^{-1} \mathbf{X}^T + \mathbf{Z}^{-1}) \mathbf{\Lambda}^T - \mathbf{\Lambda} (\mathbf{X} \mathbf{\Gamma}^{-1} \mathbf{Y}^T + \mathbf{Z}^{-1} \mathbf{\Theta}^T) - (\mathbf{Y} \mathbf{\Gamma}^{-1} \mathbf{X}^T + \mathbf{\Theta} \mathbf{Z}^{-1}) \mathbf{\Lambda}^T \right) \right) \right]
\]
\begin{align*}
&\propto \exp\left( -\frac{1}{2} \operatorname{tr} \left\{ \mathbf{\Sigma}^{-1} \left( \left( \mathbf{\Lambda} - (\mathbf{Y} \mathbf{\Gamma}^{-1} \mathbf{X}^{T} - \mathbf{\Theta} \mathbf{Z}^{-1}) (\mathbf{X} \mathbf{\Gamma}^{-1} \mathbf{X}^{T} + \mathbf{Z}^{-1})^{-1} \right) \right. \right. \right. \\
&\quad \left. \left. \left. \times (\mathbf{X} \mathbf{\Gamma}^{-1} \mathbf{X}^{T} + \mathbf{Z}^{-1}) \left( \mathbf{\Lambda} - (\mathbf{Y} \mathbf{\Gamma}^{-1} \mathbf{X}^{T} - \mathbf{\Theta} \mathbf{Z}^{-1}) (\mathbf{X} \mathbf{\Gamma}^{-1} \mathbf{X}^{T} + \mathbf{Z}^{-1})^{-1} \right)^{T} \right) \right\} \right).
\end{align*}
which implies that
\[
\mathbf{\Lambda} \mid \mathbf{\Gamma}, \mathbf{Y} \sim \mathcal{MN}\left( (\mathbf{Y} \mathbf{\Gamma}^{-1} \mathbf{X}^T - \mathbf{\Theta} \mathbf{Z}^{-1}) (\mathbf{X} \mathbf{\Gamma}^{-1} \mathbf{X}^T + \mathbf{Z}^{-1})^{-1}, \mathbf{\Sigma}, (\mathbf{X} \mathbf{\Gamma}^{-1} \mathbf{X}^T + \mathbf{Z}^{-1})^{-1} \right)
\]
\end{proof}
Note that in the special case where \(\mathbf{X} = \mathbf{I}\), i.e., a model of the form:
\[
\mathbf{Y} \mid \mathbf{\Lambda} \sim \mathcal{MN}(\mathbf{\Lambda}, \mathbf{\Sigma}, \mathbf{\Gamma})
\]
\[
\mathbf{\Lambda} \sim \mathcal{MN}(\mathbf{\Theta}, \mathbf{\Sigma}, \mathbf{Z})
\]
then the above result simplifies to
\[
\mathbf{\Lambda} \mid \mathbf{\Sigma}, \mathbf{Y} \sim \mathcal{MN}\left( (\mathbf{Y} \mathbf{\Gamma}^{-1} + \mathbf{\Theta} \mathbf{Z}^{-1}) (\mathbf{\Gamma}^{-1} + \mathbf{Z}^{-1})^{-1}, \mathbf{\Sigma}, (\mathbf{\Gamma}^{-1} + \mathbf{Z}^{-1})^{-1} \right).
\]

\section{Simulation study}
\label{sec:simulation}
\subsection{Simulation 1}
To evaluate the implementation and investigate the behavior of the MultiAddGPs model, we simulated a synthetic microbial community time-series comprising four bacterial taxa across 600 time points, based on the following model:\\
\begin{align*}
    \mathbf{f}^{(\text{periodic})}(t_n) &\sim \mathcal{MN}(0,\mathbf{\Sigma}, \mathbf{\Gamma}^{(\text{periodic})})\\
    \mathbf{f}^{(\text{trend})}(t_n) &\sim \mathcal{MN}(0,\mathbf{\Sigma}, \mathbf{\Gamma}^{(\text{trend})})  \\
    \mathbf{F}_{.n} &= 2.7 +  3x_{n}^{(\text{batch})} + \mathbf{f}^{(\text{periodic})}(t_n) + \mathbf{f}^{(\text{trend})}(t_n)\\
    \boldsymbol{\Pi}_{.n} &= ALR^{-1}(\mathbf{H})\\
    \mathbf{Y}_{.n} &\sim \text{Multinomial}(\mathbf{\Pi}_{.n})\\
\end{align*}
Here, we set $\mathbf{\Sigma}$ as a covariance matrix with off-diagonal elements of 0.9 and diagonal elements of 1.5. The periodic kernel is defined as $\mathbf{\Gamma}^{(\text{periodic})} = 4 \exp\left(-\frac{2 \sin^2\left(\frac{\pi |t - t'|}{25}\right)}{30^2}\right)$, while the trend kernel is modeled as $\mathbf{\Gamma}^{(\text{trend})} = \exp\left(-\frac{(t - t')^2}{2 \times 30^2}\right)$. After obtaining the posterior samples from the MultiAddGPs model, we apply a sum-to-zero constraint to facilitate model identification.

In Figure 1 of the main text, we illustrate the model's ability to successfully decompose the simulated microbiome time-series for a single taxon. In Figures \ref{fig: Taxa2} and \ref{fig: Taxa3} in the supplementary section, we further demonstrate this decomposition for two additional taxa.

Next, we assessed the scalability of the model. However, as the dimensions ($D$) and number of time points ($N$) increased, it became increasingly challenging to simulate data with a distinct non-linear trend suitable for additive modeling. To address this, we replaced the non-linear trend kernel $\mathbf{\Gamma}^{(trend)}$ with a linear kernel: $\mathbf{\Gamma}^{(trend)} = 20^2 + (t - c)(t' - c)$, while keeping the rest of the model unchanged. We then simulated this modified model across various combinations of $D$ and $N$, where $D \in {3, \dots, 100}$ and $N \in {50, \dots, 1000}$. For each combination of $(D, N)$, we generated three simulated datasets. The coverage ratio, presented in Figure 2 of the main text, represents the average across these three simulations.

Analysis of the simulated dataset revealed that the estimates for the unobserved compositions, $\mathbf{H}$, and latent factors, $\mathbf{F}$, obtained from the MultiAddGPs model were more accurate compared to those derived from the standard approach of normalizing read counts to proportions (NAddGPs). Furthermore, our model successfully disentangled distinct effects arising from multiple linear and non-linear factors. These results suggest that our model is capable of effectively decomposing longitudinal microbiota data into a mixture of linear and non-linear additive components.

All implements were compiled and run using gcc version 9.1.0 and R version 4.3.2. All replicates of the simulated count data were supplied to the various implementions independently and the models were fit on identical hardware, allotted 64GB RAM, 4 cores, and restricted to a 48-hour upper limit on run-time.

\begin{figure}[H]
    \centering
    \includegraphics[width=1\linewidth]{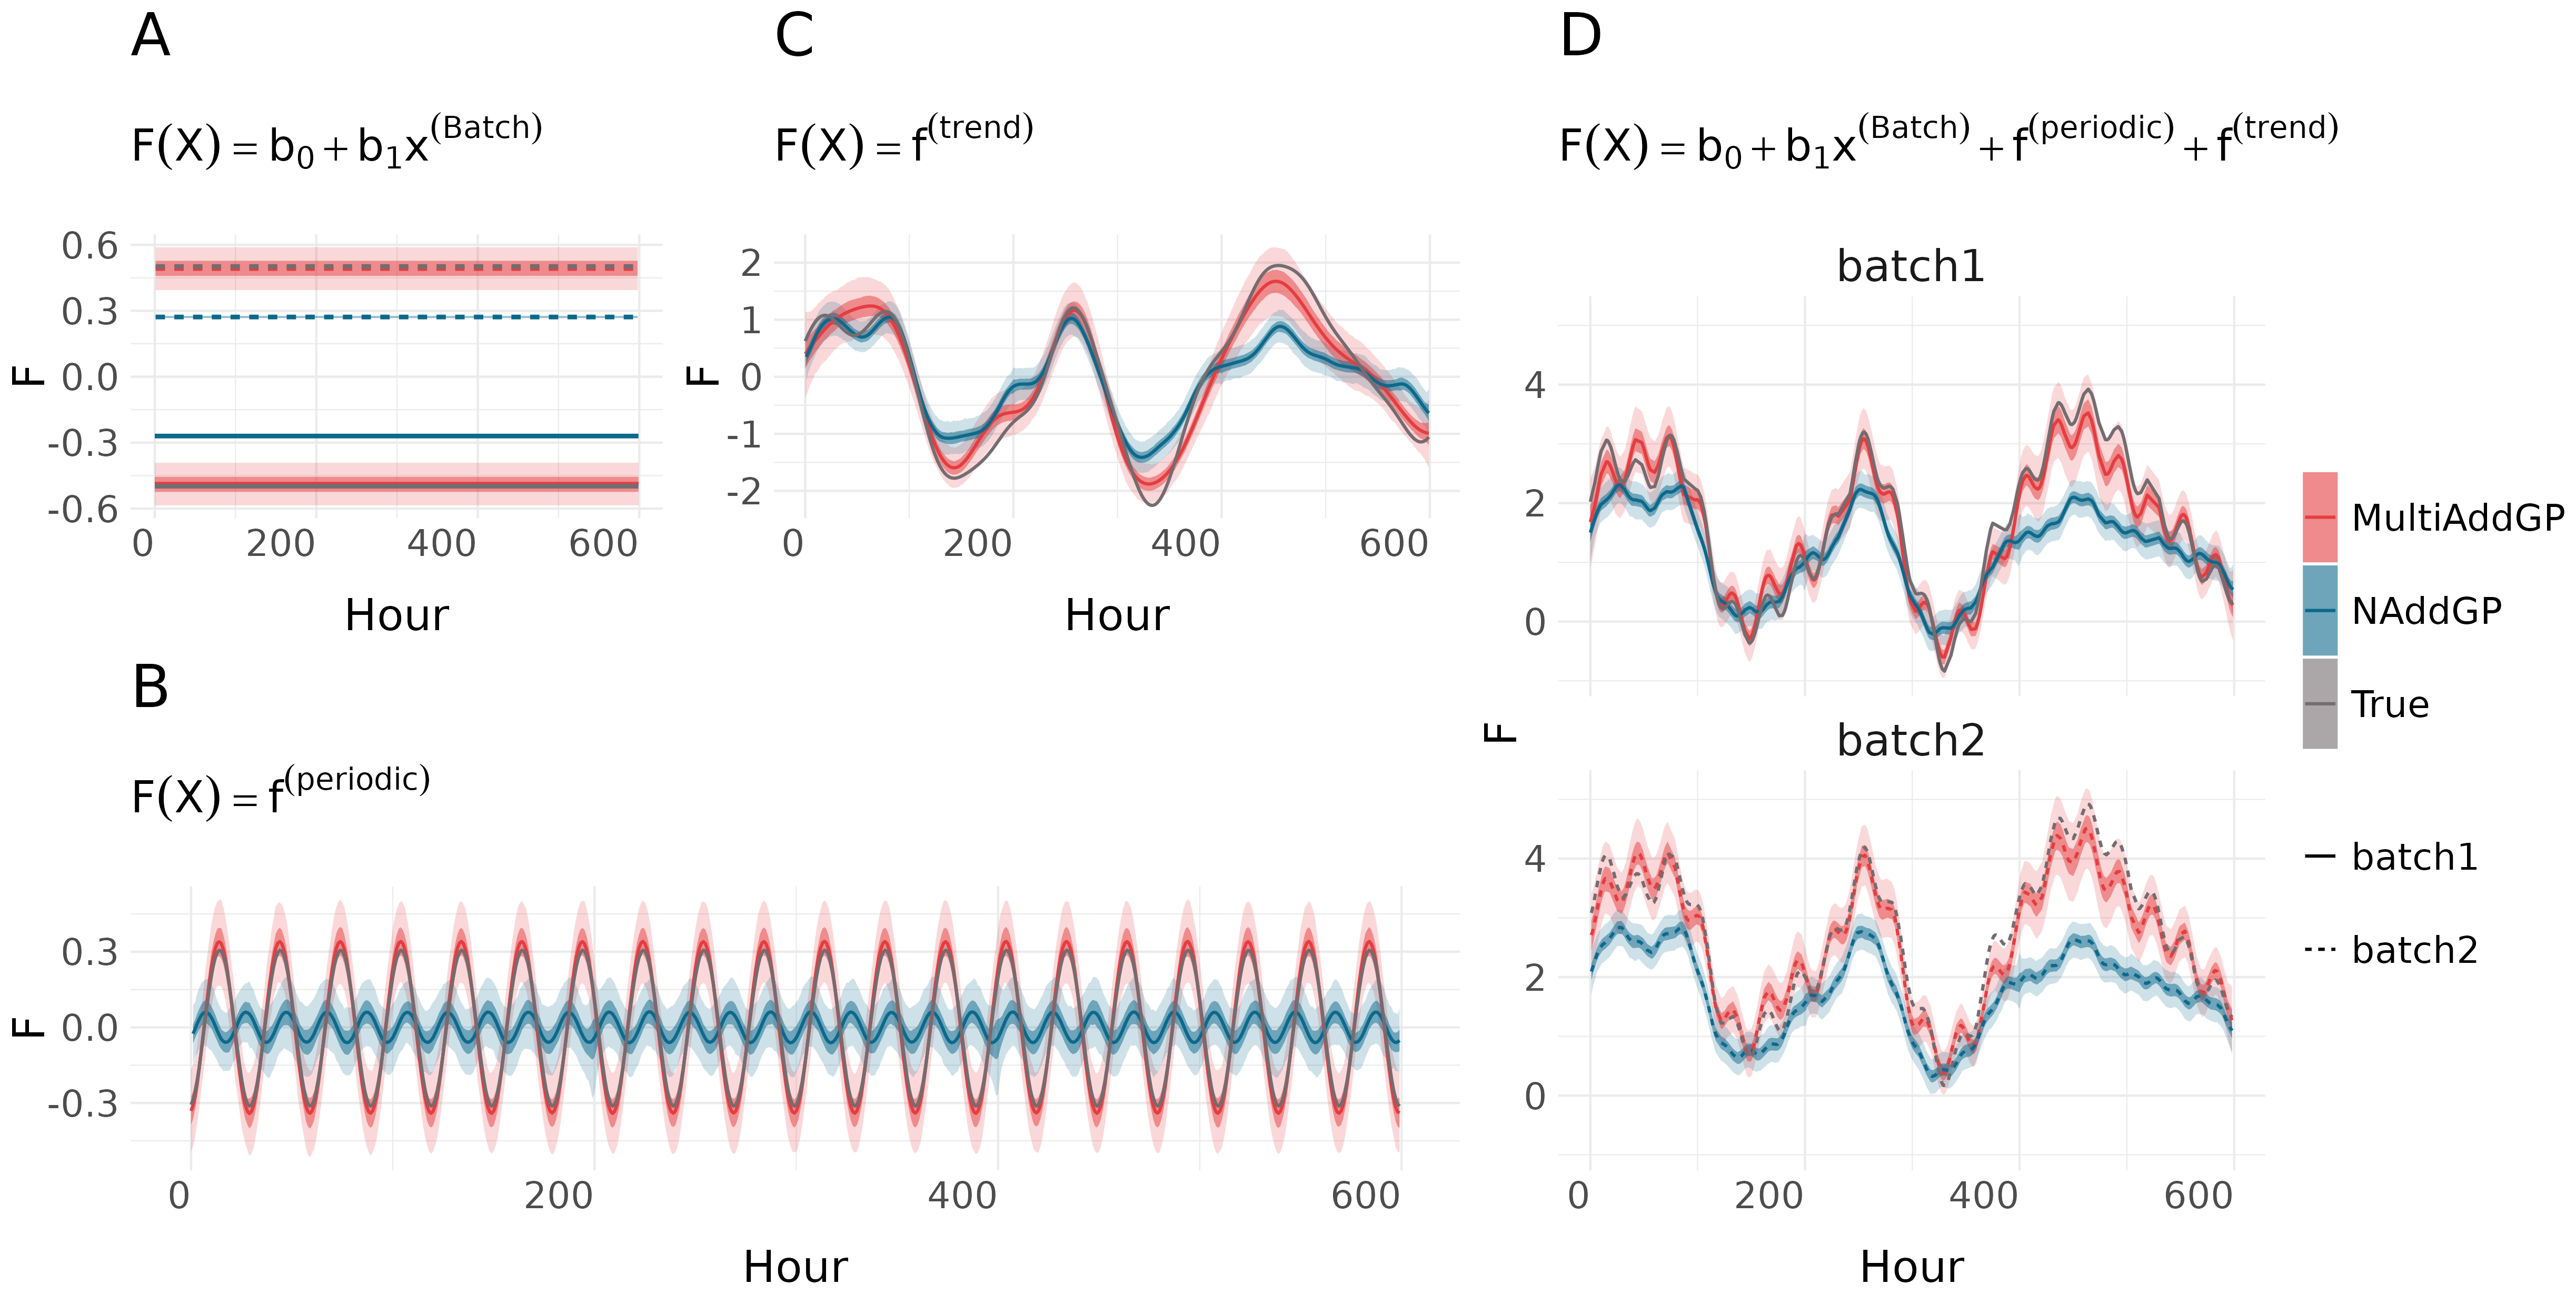}
    \caption{MultiAddGPs successfully decompose simulated microbiome time-series on Taxa 2.}
    \label{fig: Taxa2}
\end{figure}

\begin{figure}[H]
    \centering
    \includegraphics[width=1\linewidth]{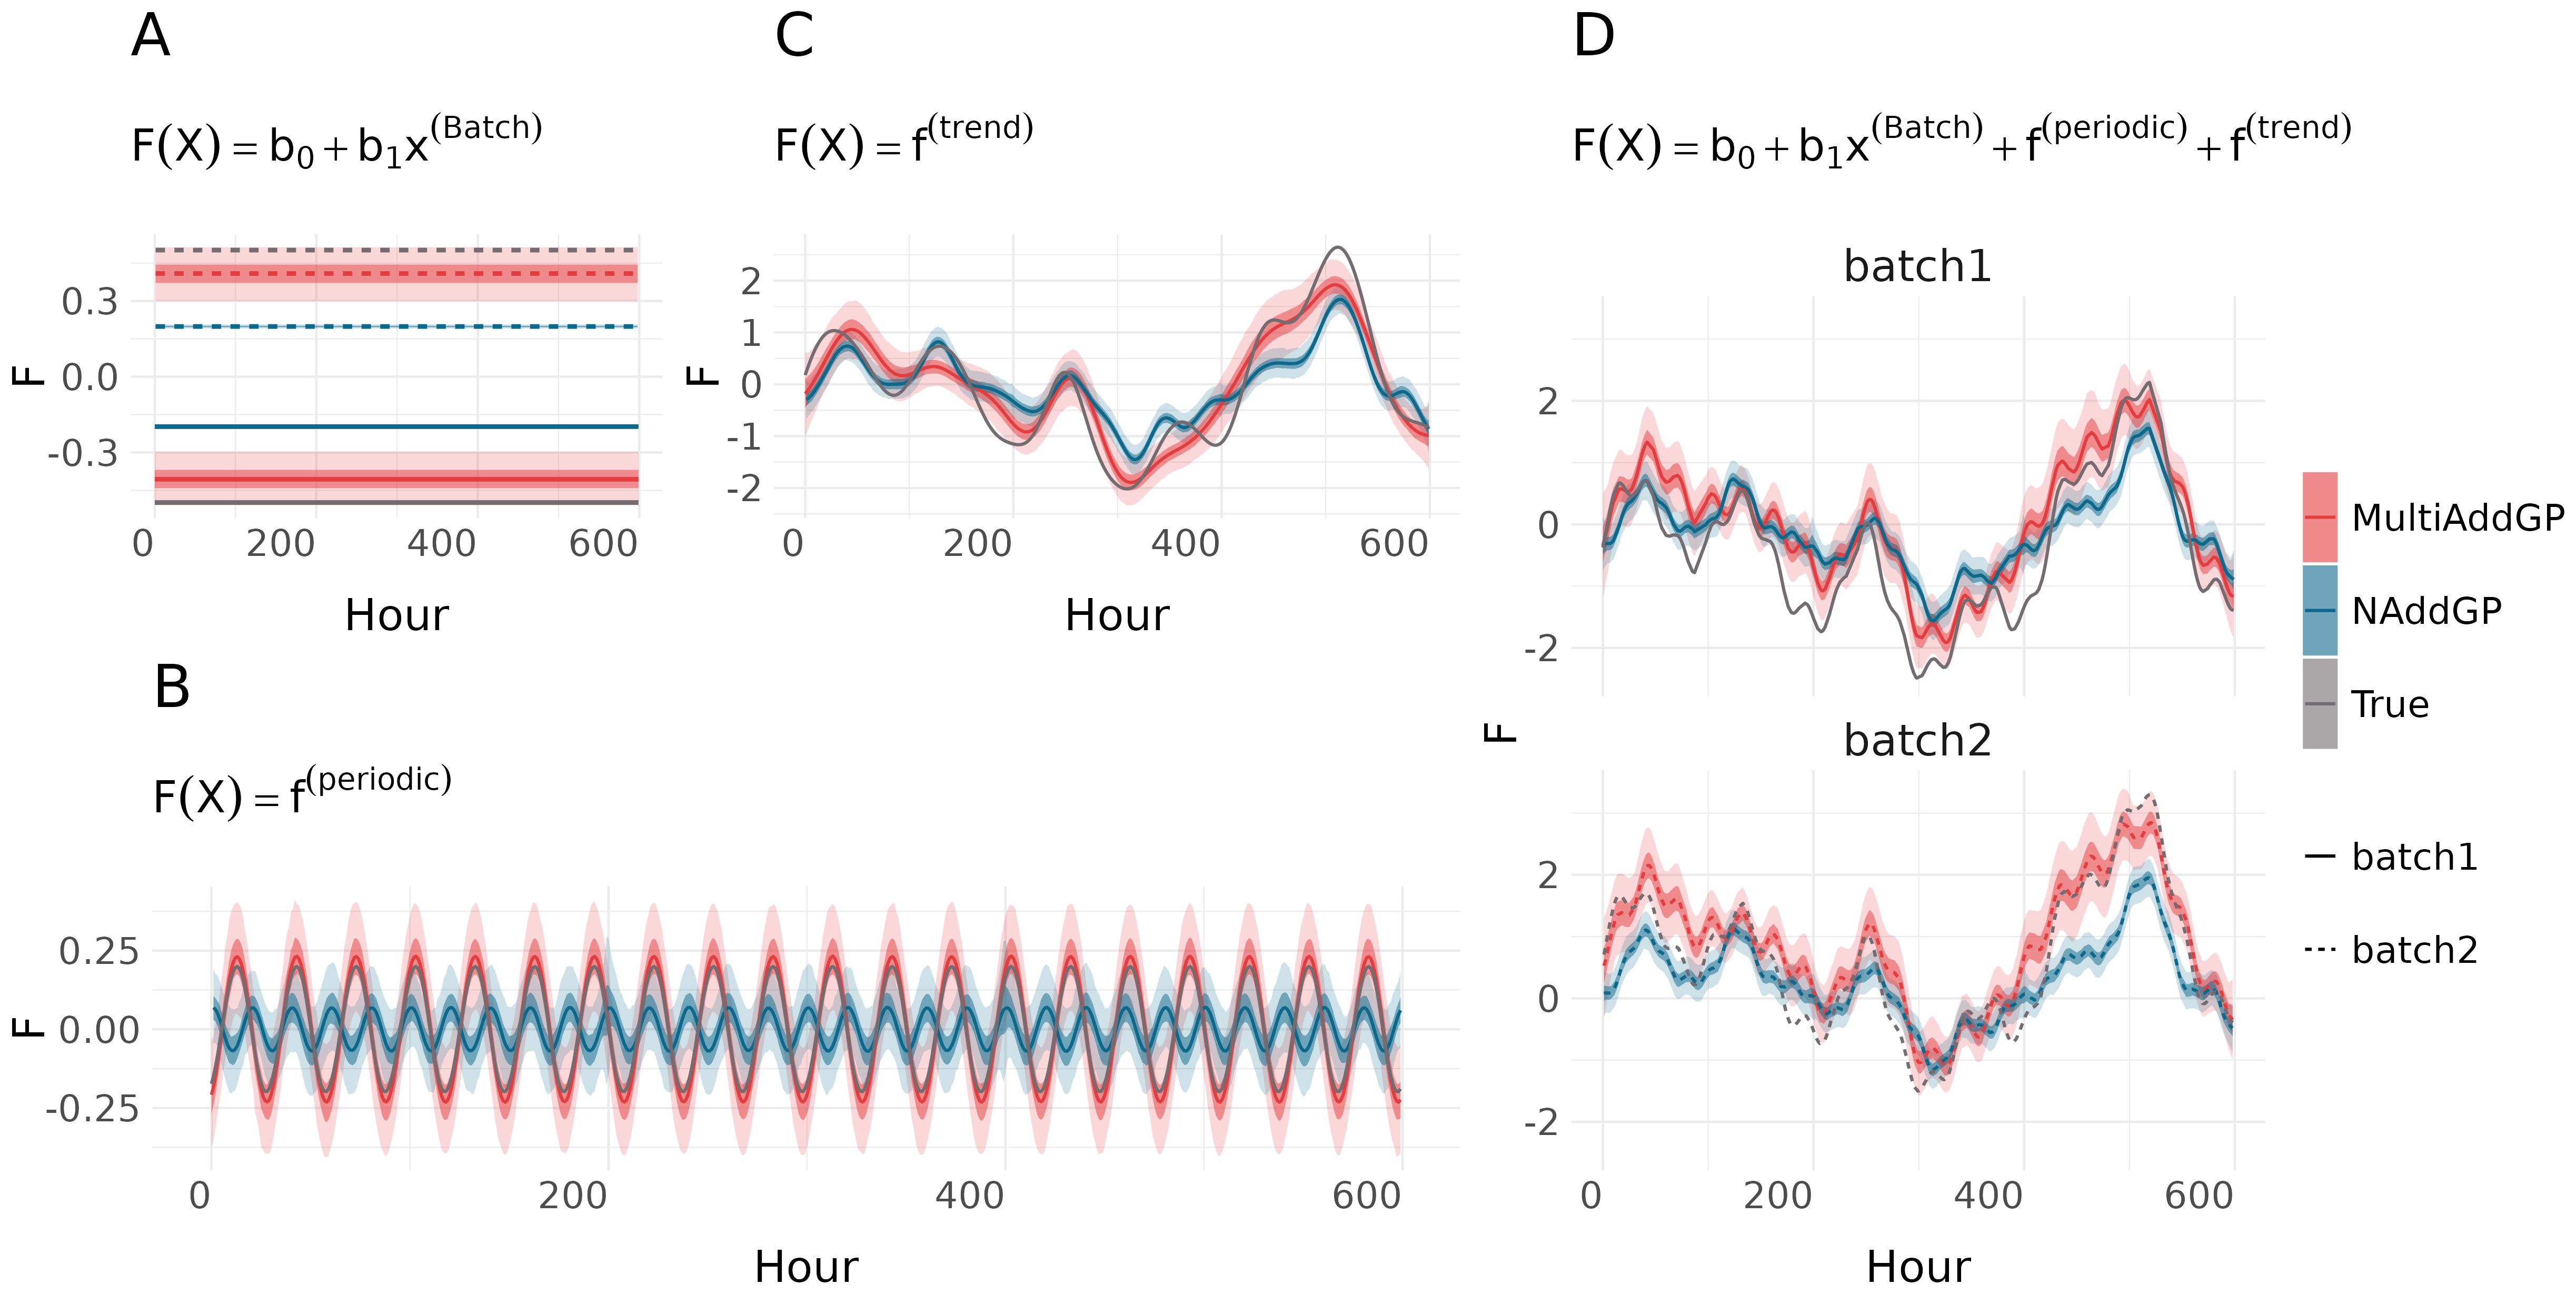}
    \caption{MultiAddGPs successfully decompose simulated microbiome time-series on Taxa 3.}
    \label{fig: Taxa3}
\end{figure}

\subsection{Simulation 2} To evaluate the performance of our model relative to the existing method \textit{Lgpr} \citep{timonen2021lgpr}, we conducted a simulation study. Since Lgpr does not scale to larger datasets, we generated a small dataset with 
with $D = 3$ and $N = 50$ for inference comparison. The simulation follows the model:
\begin{align*}
\mathbf{f}^{(\text{non-stationary})}(w_n) &\sim \mathcal{MN}(0,\mathbf{\Sigma}, \mathbf{\Gamma}^{(\text{non-stationary})})\\
\mathbf{f}^{(\text{trend})}(t_n) &\sim \mathcal{MN}(0,\mathbf{\Sigma}, \mathbf{\Gamma}^{(\text{trend})}) \\
\mathbf{F}{.n} &= 0.4 + x_{n}^{(\text{batch})} + \mathbf{f}^{(\text{non-stationary})}(w_n) + \mathbf{f}^{(\text{trend})}(t_n)\\
\boldsymbol{\Pi}{.n} &= ALR^{-1}(\mathbf{H})\\
\mathbf{Y}{.n} &\sim \text{Multinomial}(\mathbf{\Pi}_{.n})
\end{align*}
Here,  $w_n$ is a transformed skewed Gaussian of input $t_n$, used in the non-stationary kernel model:
\begin{align*}
z_n &= \frac{t_n - m}{s}\\
w_n &= \exp\left(\frac{1}{2}z_n^2\right) \times \frac{1}{1+ \exp(-\alpha z_n)} \end{align*}
where $m$ determines the peak location of the distribution, $s$ controls its width, and $\alpha$ is the skew parameter. When 
$\alpha = 0$, the function reduces to a standard Gaussian; positive $\alpha$ induces a heavier right tail, while negative $\alpha$ results in a heavier left tail. In this simulation, the covariance matrix $\Sigma$ is set with off-diagonal elements of 0.5 and diagonal elements of 1. The non-stationary kernel is defined as $\mathbf{\Gamma}^{(\text{non-stationary})}= 2 \times \text{exp}(-\frac{(t-t')^2}{2 \times 3^2})$ , while the general kernel is modeled as $\mathbf{\Gamma}^{(\text{trend})}= \text{exp}(-\frac{(t-t')^2}{2 \times 0.5^2})$. As in Simulation 1, we apply a sum-to-zero constraint to facilitate model identification after obtaining posterior samples from both models.

Since Lgpr utilizes predefined kernels, we aimed to select the most appropriate kernel configurations to closely align with their model structure. The Lgpr model was fitted using the lgp function with a structured formula. Specifically, the response variable $Y$ was modeled as a function of an interaction term between zero-sum kernel: $zs(\text{ID})$ and a Gaussian process over time: $gp(t_n)$, designed to capture long-term temporal trends. To model batch effects, we employed their sum-zero kernel for categorical variables, $zs(x_n^{\text{batch}})$. $gp\_ns(t_n)$ was used for modeling the non-stationary effect. A negative binomial ("nb") likelihood was specified, and the prior distribution were set as follows:a normal prior $\mathcal{N}(2,1)$ for the $\alpha$ parameter, a normal prior $\mathcal{N}(0.8,1)$ for the length scale $\ell$, and a log-normal prior $\text{log}\mathcal{N}(1,1)$ for the warping parameter. The model was trained using 5000 iterations across 4 MCMC chains, with a refresh interval of 2000. To improve sampling efficiency, the control settings included an adaptation delta of 0.999 and a maximum tree depth of 11. 

\begin{figure}[H]
    \centering
    \includegraphics[width=1.1\linewidth]{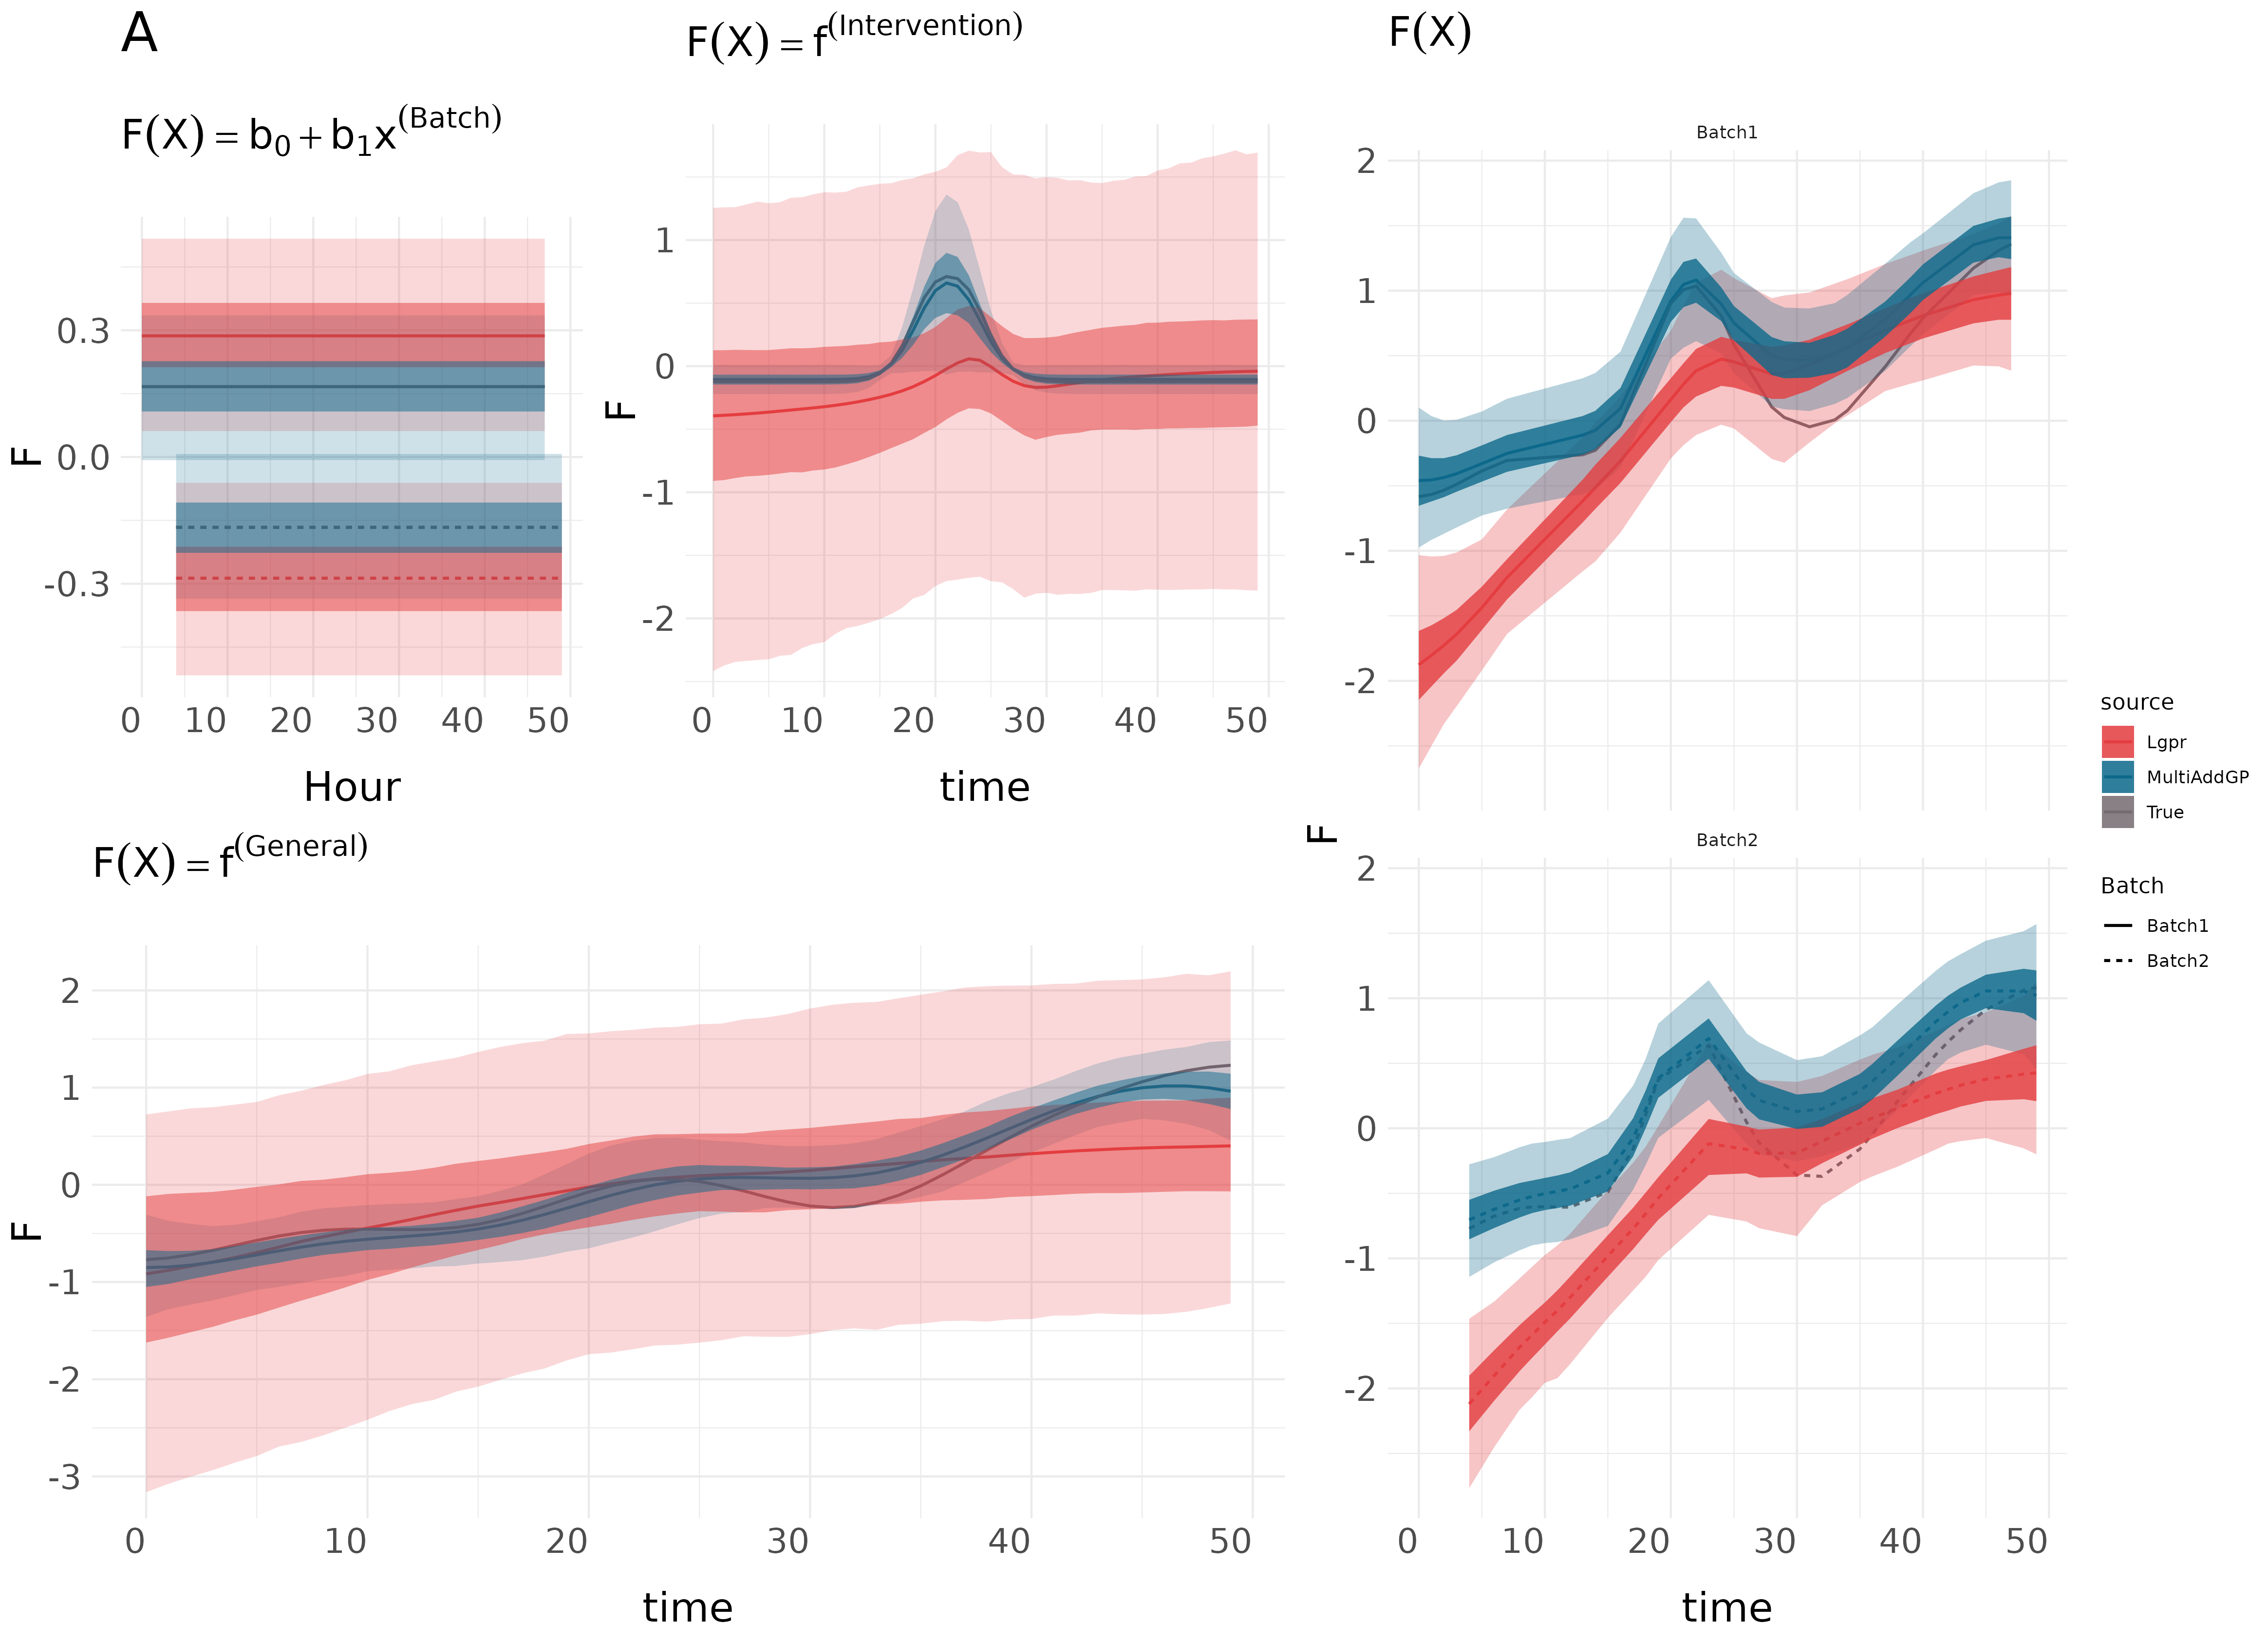}
    \caption{Inference comparison between MultiAddGPs and Lgpr}
    \label{fig: inference_com}
\end{figure}

Figure \ref{fig: inference_com} presents the inference performance of the two models in Simulation 2. While the uncertainty estimates of the Lgpr model include the true values, the associated uncertainty is excessively wide, which makes it ineffective in capturing the underlying pattern and providing meaningful insights. In contrast, MultiAddGPs accurately capture the true pattern with significantly lower uncertainty. Notably, the Lgpr model required approximately 7 hours to complete the analysis for a single taxon, whereas MultiAddGPs performed the same analysis for all taxa in under one minute.

\section{Details on Artificial gut data application}
\label{sec:artificial}

We describe the specific MultiAddGPs model applied to the artificial gut dataset as a particular instance of the broader MultiAddGPs framework. Simplifications were introduced in three key areas: model structure, kernel selection, and prior specification.

First, regarding model structure, we analyzed four concurrent time series from four artificial gut vessels. Given that the primary goal of our modeling was to isolate the effect of feed disruption, we represented the data as comprising two overlapping temporal processes: a vessel-specific long-term trend, $\mathbf{f}^{(\text{base},v)}$, and a vessel-specific function capturing the effect of starvation, $\mathbf{f}^{(\text{disrupt},v)}$. Moreover, as the vessels were physically isolated from each other, we modeled them as independent processes by using block identity matrices $\mathbf{\Gamma}^{(v)}$ such as:
\begin{align*}
    \mathbf{\Gamma}^{(v)} \odot \mathbf{\Gamma}^{(\text{base})} =  \begin{bmatrix}
                                                    \mathbf{\Gamma}^{(v=1,\text{base})} & 0 & 0 & 0 \\
                                                    0  & \mathbf{\Gamma}^{(v=2,\text{base})} & 0 & 0\\
                                                    0 & 0 & \mathbf{\Gamma}^{(v=3,\text{base})}  & 0\\
                                                    0 & 0 & 0 &\mathbf{\Gamma}^{(v=4,\text{base})}
                                                  \end{bmatrix}
\end{align*}
\begin{align*}
    \mathbf{\Gamma}^{(v)} \odot \mathbf{\Gamma}^{(\text{disrupt})} =  \begin{bmatrix}
                                                    \mathbf{\Gamma}^{(v=1,\text{disrupt})} & 0 \\
                                                    0  & \mathbf{\Gamma}^{(v=2,\text{disrupt})}\\
                                                  \end{bmatrix}
\end{align*}
as the covariance structure of $\mathbf{f}^{(\text{base},v)}$ and $\mathbf{f}^{(\text{disrupt},v)}$,  where $\odot$ represents the Kronecker product. To simplify prior specification, we standardized all continuous covariates (before fitting to the model) so that their means were zero and their standard deviations were one.

All prior mean functions were set to the zero function. We use a squared exponential kernel to model long-term non-linear trends in $\mathbf{\Gamma}^{(\text{base})}$:
$$\mathbf{\Gamma}^{(\text{base})} = \sigma_{\text{base}}^2 \exp\left(- \frac{(t_n-t_n')^2}{2 \rho_{\text{base}}^2}\right)$$
For the disruption effects, we employ a rational quadratic kernel set to zero prior to day 11. This reflect the assumption that the target variable exhibits varying degrees of smoothness and irregularities near or after the starvation period:
$$\mathbf{\Gamma}^{(\text{disrupt})} = \sigma_{\text{disrupt}}^2 \left(1+\frac{(t_n-t_n')^2}{2a \rho_{\text{disrupt}}^2}\right)^{-a}\mathbf{I}(t_n\geq 11\, \&\, t_n'\geq 11).$$
Regarding the prior settings for the hyperparameters, we specified two types of prior distributions for the parameters in the kernel functions: the prior over the length scale parameters ($\rho_{\text{base}}, \rho_{\text{disrupt}}$) and the magnitude parameters ($\sigma_{\text{base}}, \sigma_{\text{disrupt}}$) of the kernel. For both sets of parameters in each kernel, we adopted an InverseGamma distribution as follows:
\begin{align*} \rho_{\text{base}}, \rho_{\text{disrupt}} &\sim \text{InverseGamma}(\alpha_1, \beta_1) \\
\sigma_{\text{base}}, \sigma_{\text{disrupt}} &\sim \text{InverseGamma}(\alpha_2, \beta_2) \end{align*}
with $\alpha_1 = 10$, $\beta_1 = 20$, $\alpha_2 = 10$, $\beta_2 = 10$ for $\mathbf{\Gamma}^{(\text{base})}$, and $\alpha_1 = 10$, $\beta_1 = 10$, $\alpha_2 = 10$, $\beta_2 = 20$ for $\mathbf{\Gamma}^{(\text{disrupt})}$ (see Figure \ref{fig:priordensity} for density plot). Note that we fixed the $a$ parameter in the rational quadratic kernel, which determines the relative weighting of large-scale and small-scale variations, at a value of 2. These specification reflects our assumption that the model is constrained from learning distances that are significantly smaller or larger than the temporal distances among $t$. In other words, the prior penalizes extremely small or large length scales. The penalized marginal likelihood is given by
\begin{align*}
  \label{eq:laplace-approx-marginallikelihood_penalty1} 
  \log \int p(\pmb{H}, \pmb{Y} \mid  \Omega) d\pmb{H} & \approx \frac{(D-1)N}{2}\log(2\pi) +  \log p(\hat{\mathbf{H}}_{\Omega}, \mathbf{Y} \mid  \Omega)-\frac{1}{2} \log (|\nabla^2[vec(\hat{\mathbf{H}}_{\Omega})]|)\\
   &\quad + \lambda \times [\log p(\rho_{\text{base}})+ \log p(\rho_{\text{disrupt}}) +\log p(\sigma_{\text{base}})+ \log p(\sigma_{\text{disrupt}})].
\end{align*}
To aid in model identification, we also imposed the constraint $\sigma_{\text{base}} < \sigma_{\text{disrupt}}$, assuming greater variation is attributed to the starvation kernel following prior resports~\cite{silverman2018dynamic}. Finally, we set $\rho_{\text{base}} > \rho_{\text{disrupt}}$, reflecting the expectation that, in the absence of starvation, the base kernel should exhibit smoother and flatter trends. Note that we did not center the posterior samples at a mean of 0, as no intercept was included in the model.
We chose \(\lambda=120\) which was the smallest value of that was able to identify the distinction between \(\mathbf{f}^{(\text{disrupt})}\) and \(\mathbf{f}^{(\text{base})}\). No perceptible change in estimated disruption effects was observed for values between 120 and 200. 

\begin{figure}[H]
    \centering
    \includegraphics[width=\linewidth]{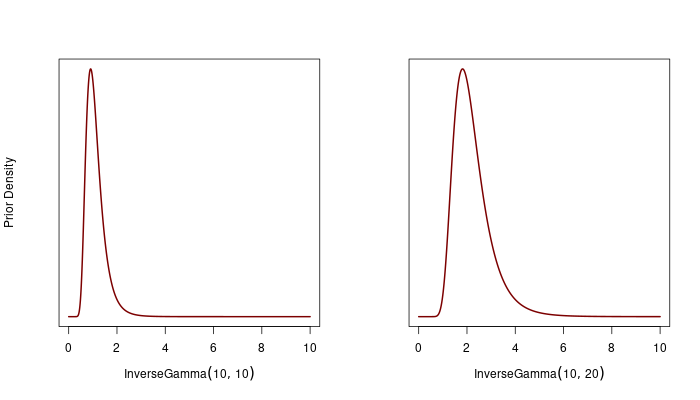}
    \caption{Prior density plots for the InverseGamma distributions used for the hyperparameters in the kernel functions (Artificial gut data)}
    \label{fig:priordensity}
\end{figure}

\section{Details on Lifestyle microbiome data} 
We describe the application of MultiAddGPs to the longitudinal microbiome dataset. Compared to the artificial gut data, this study involves a simpler model structure with only one single time series. However, it still captures two overlapping temporal processes: a general long-term trend, $\mathbf{f}^{\text{(trend)}}$, and a travel intervention effect, $\mathbf{f}^{\text{(travel)}}$, which induces rapid microbiome fluctuations. The time series was standardized to have a mean of zero and a standard deviation of one before model fitting. All kernel mean functions were set to zero, and both temporal components were modeled using squared exponential kernels:
\begin{align*} \mathbf{\Gamma}^{(\text{trend})} &= \sigma_{\text{trend}}^2 \exp\left(-\frac{(t_n-t_n')^2}{2\rho_{\text{trend}}^2}\right), \\
\mathbf{\Gamma}^{(\text{travel})} &= \sigma_{\text{travel}}^2 \exp\left(-\frac{(w(t_n)-w(t_n)')^2}{2\rho_{\text{travel}}^2}\right). \end{align*}

Here,  $w(t_n)$ is a transformed skewed Gaussian of input $t_n$, designed to capture the non-stationary nature of the travel intervention. Specifically:
\begin{align*}
z_n &= \frac{t_n - m}{s}\\
w_n &= \exp\left(\frac{1}{2}z_n^2\right) \times \frac{1}{1+ \exp(-\alpha z_n)} \end{align*}
where $m$ determines the peak location of the distribution, $s$ governs its width, and $\alpha$ is the skew parameter. When 
$\alpha=0$, the function reduces to a standard Gaussian; a positive value of $\alpha$ induces a heavier right tail, while negative value produce a heavier left tail.  Here we set $m=92$, $s=20$, and $\alpha=2$. These choices effectively restrict the travel-related changes to a two-month window after the travel date, ensuring that the model captures the local, non-stationary fluctuations associated with travel without introducing undue influence at other time points.

For the kernel hyperparameters, we specified the following prior distributions:
\begin{align*} \sigma_{\text{trend}}, \sigma_{\text{travel}}, \rho_{\text{travel}} &\sim \mathcal{N}(5,1),\\
\rho_{\text{trend}} &\sim \text{InverseGamma}(10,0.8). \end{align*}
This specification reflects prior knowledge from previous studies \cite{david2014host}, suggesting that the long-term microbiome trend is more stable, while travel-induced changes exhibit greater variation and sharper fluctuations. In other words, the prior penalizes extremely small or large length scales. The penalized marginal likelihood is given by
\begin{align*}
  \log \int p(\pmb{H}, \pmb{Y} \mid  \Omega) d\pmb{H} & \approx \frac{(D-1)N}{2}\log(2\pi) +  \log p(\hat{\mathbf{H}}_{\Omega}, \mathbf{Y} \mid  \Omega)-\frac{1}{2} \log (|\nabla^2[vec(\hat{\mathbf{H}}_{\Omega})]|)\\
   &\quad + \lambda \times [\log p(\rho_{\text{trend}})+ \log p(\rho_{\text{travel}}) +\log p(\sigma_{\text{trend}})+ \log p(\sigma_{\text{travel}})].
\end{align*}

To ensure model identifiability, we imposed the constraints $\sigma_{\text{trend}} < \sigma_{\text{travel}}$ and $\rho_{\text{trend}} > \rho_{\text{travel}}$, reflecting the assumption that the travel-related kernel captures higher-frequency variation, while the general trend evolves more smoothly and gradually. The posterior distributions were centered at a mean of zero. The full set of posterior estimates for the bacterial family-level contributions of $\mathbf{f}^{\text{trend}}$, $\mathbf{f}^{\text{travel}}$, and their cumulative effect $\mathbf{f}^{\text{trend}} + \mathbf{f}^{\text{travel}}$ are presented in Figures~\ref{fig:Long_trend},\ref{fig:Long_travel}, and \ref{fig:long_F}.

\begin{figure}[H]
    \centering
    \includegraphics[width=\linewidth]{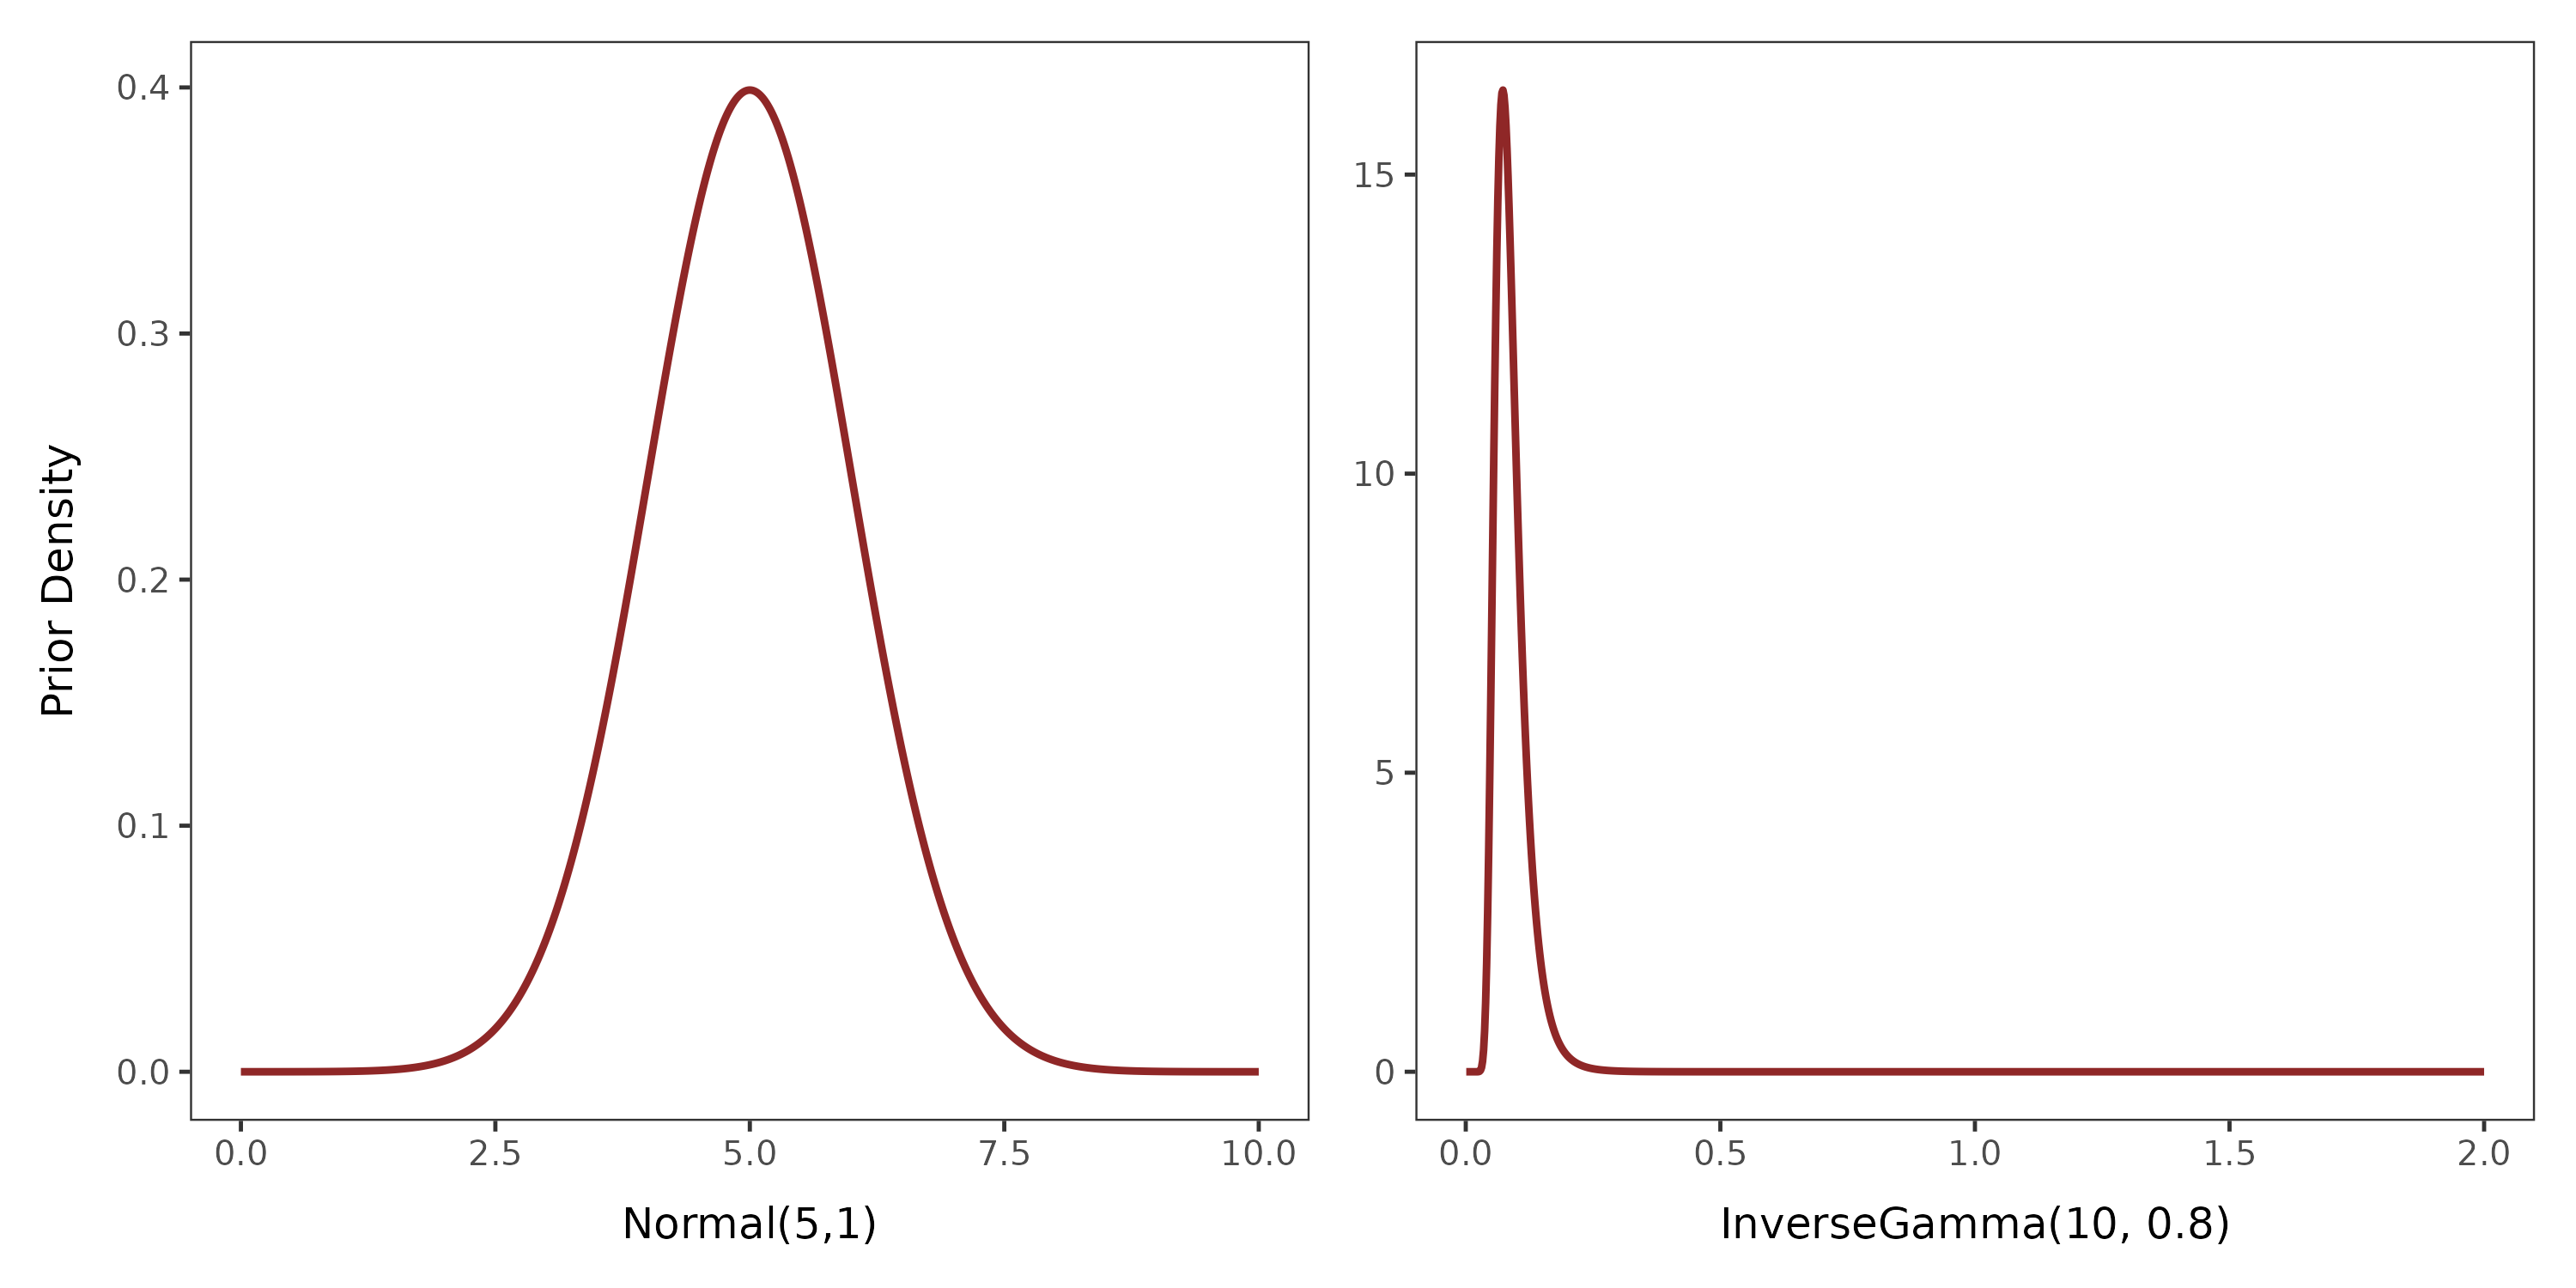}
    \caption{Prior density plots for the Normal and InverseGamma distributions used for the hyperparameters in the kernel functions (Longitudinal microbiome data).}
    \label{fig:prior_longitudinal}
\end{figure}

\begin{figure}[H]
     \centering
    \includegraphics[width=15cm]{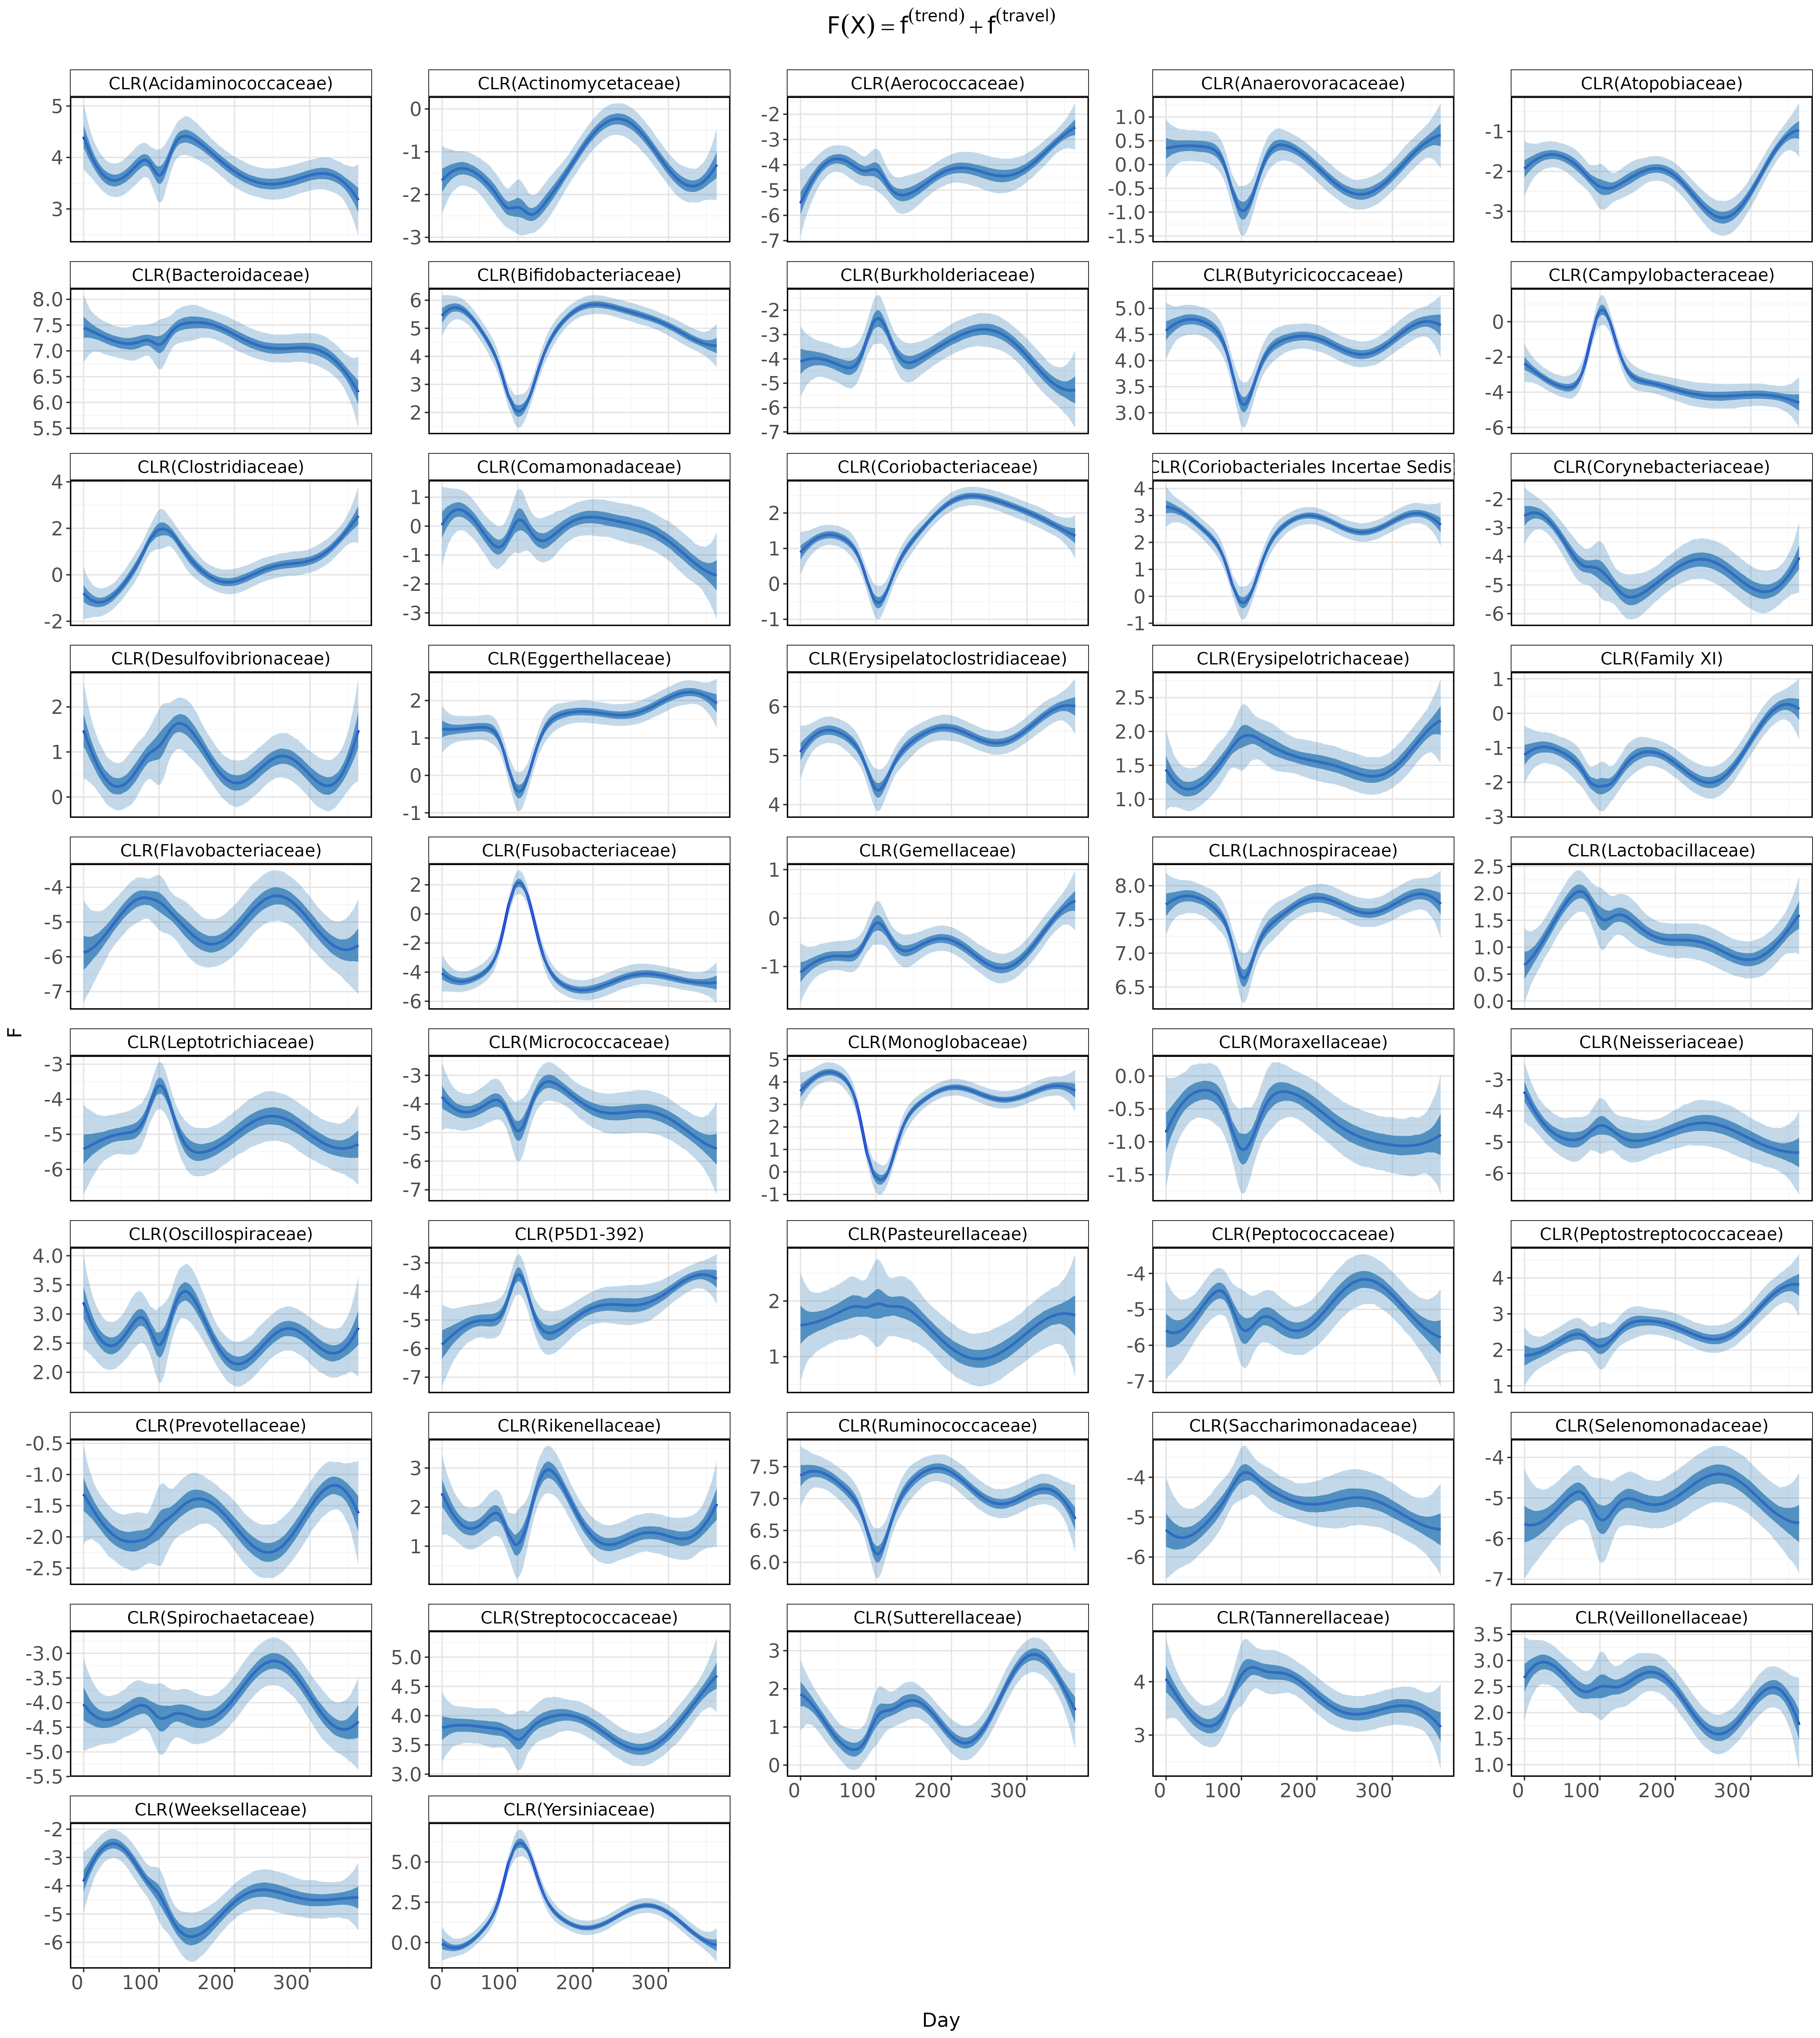}
    \caption{MultiAddGPs Posterior for the Smoothed State F in the Longitudinal Microbiome Study}
    \label{fig:long_F}
\end{figure}
\newpage

\begin{figure}[H]
     \centering
    \includegraphics[width=15cm]{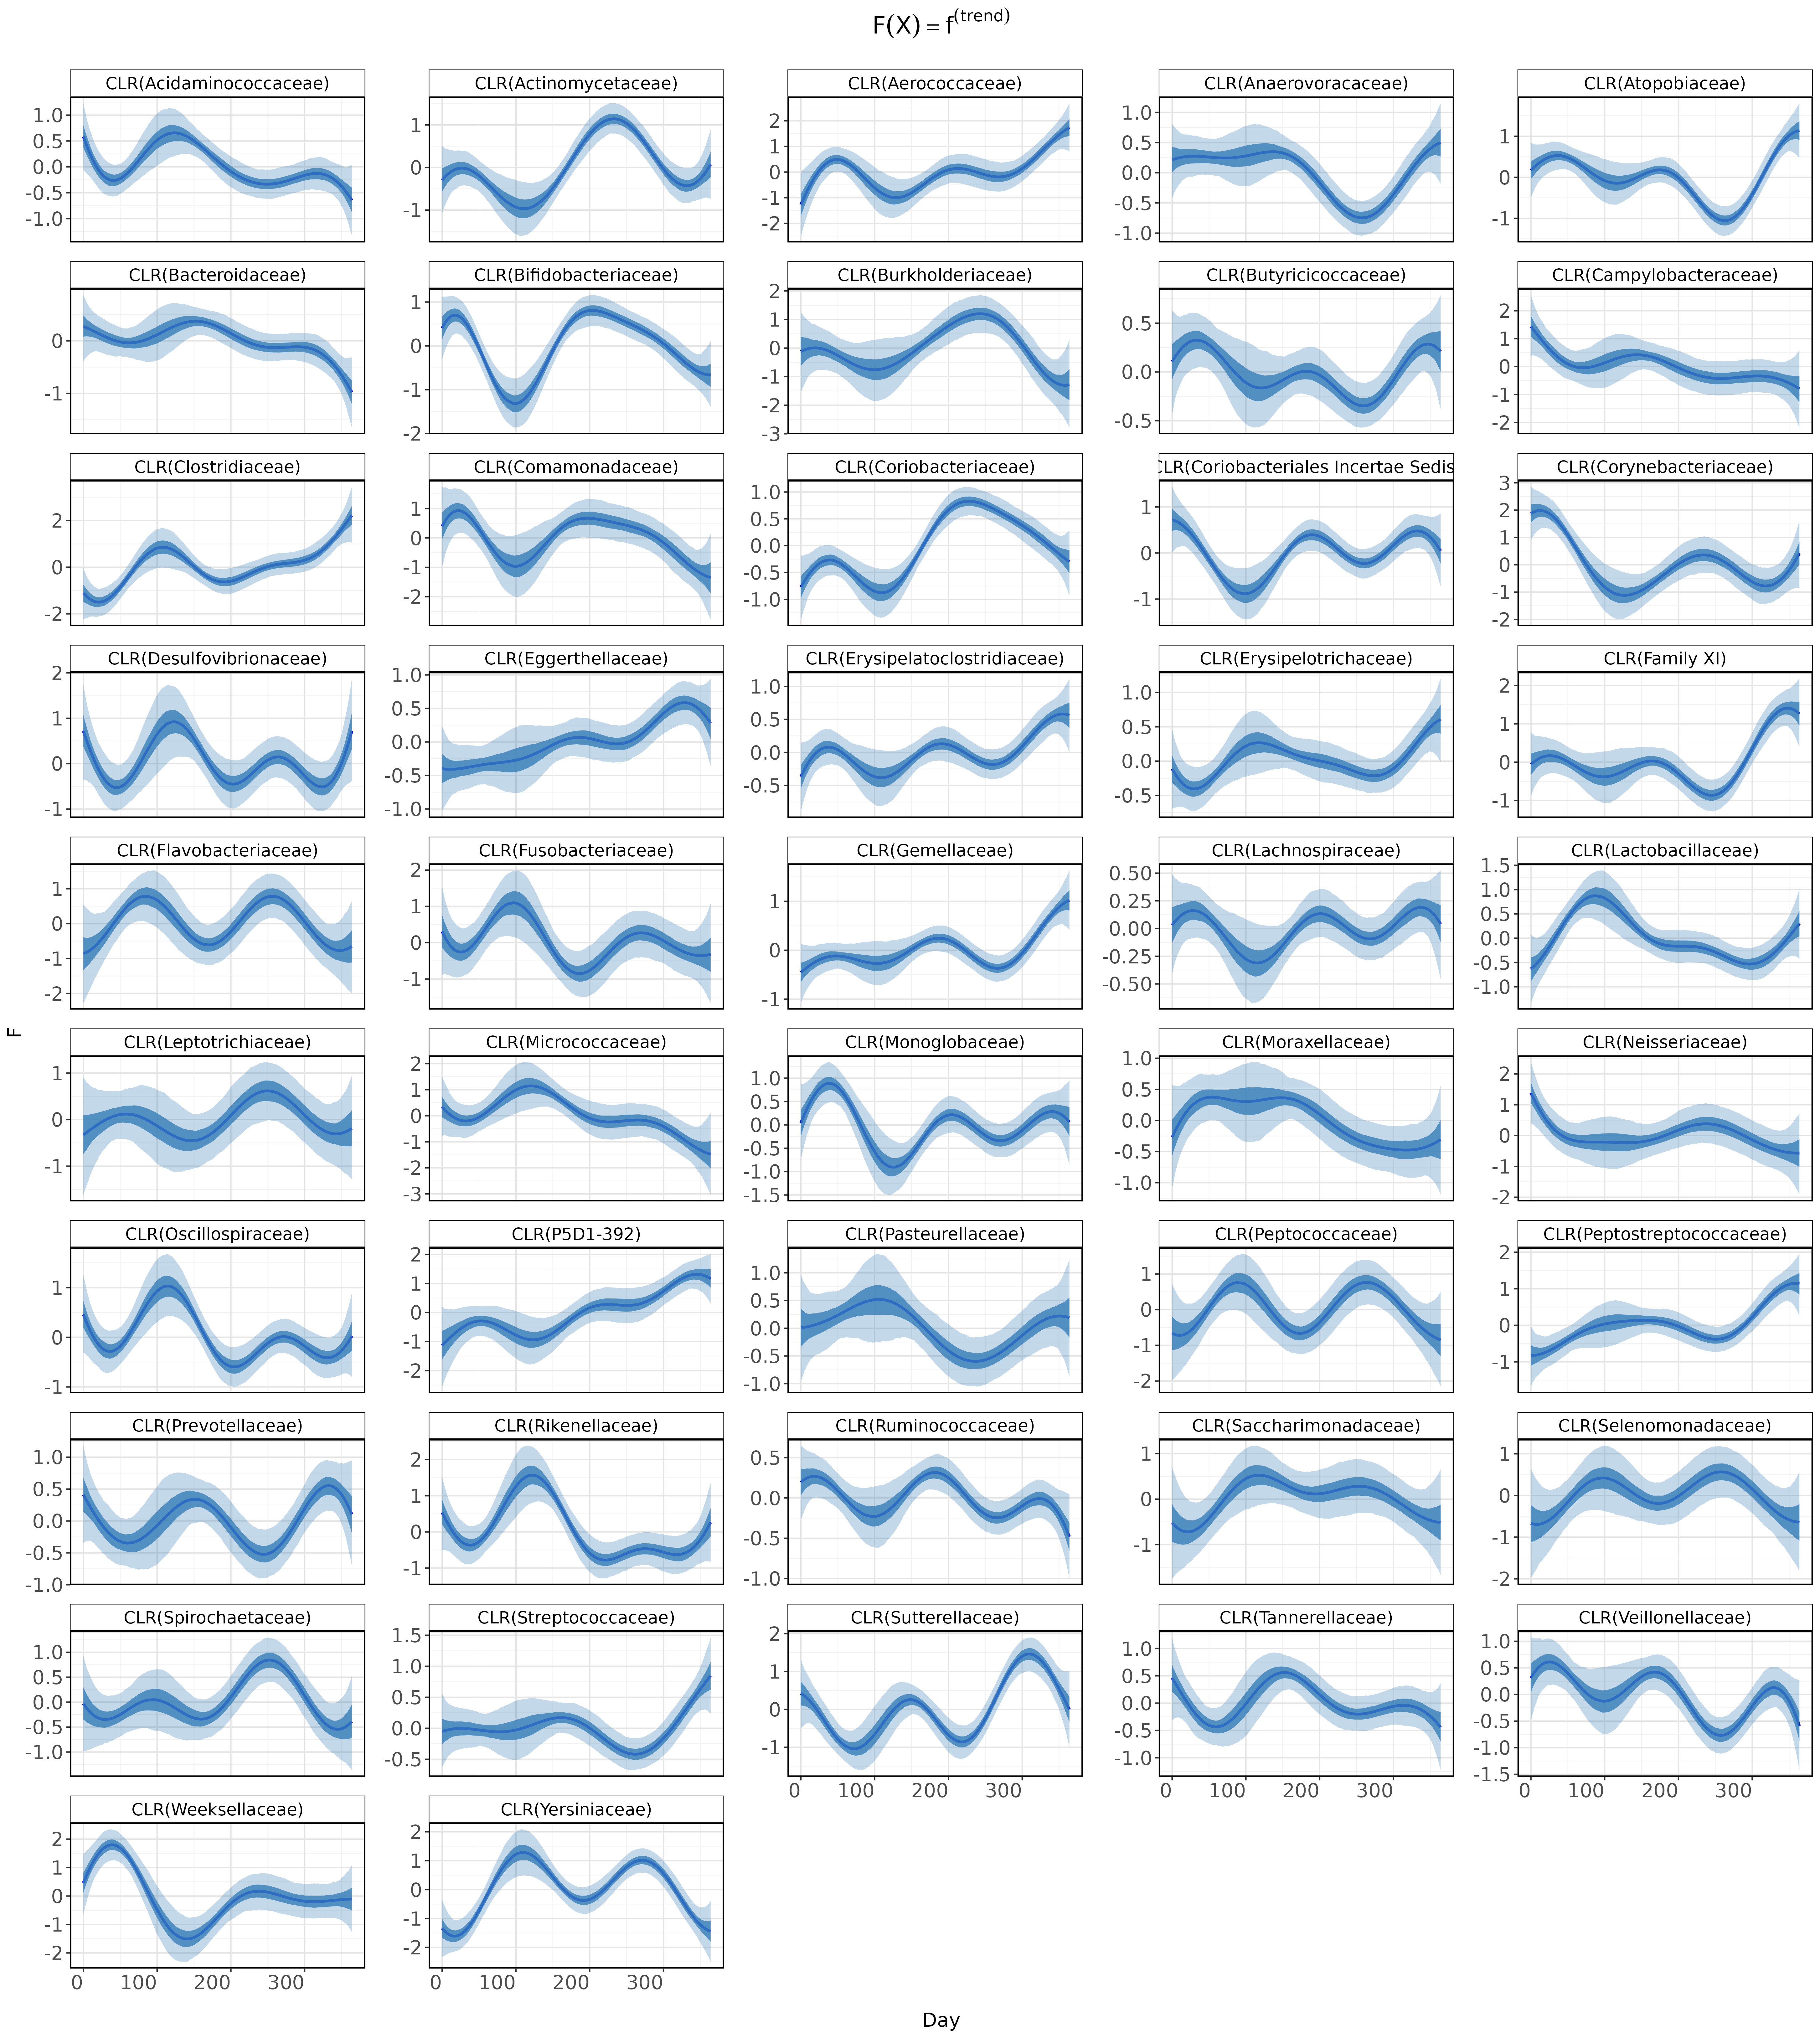}
    \caption{MultiAddGPs Posterior for the general trend effect $\mathbf{f}^{\text{(trend)}}$ in the Longitudinal Microbiome Study}
    \label{fig:Long_trend}
\end{figure}
\newpage

\begin{figure}[H]
     \centering
    \includegraphics[width=15cm]{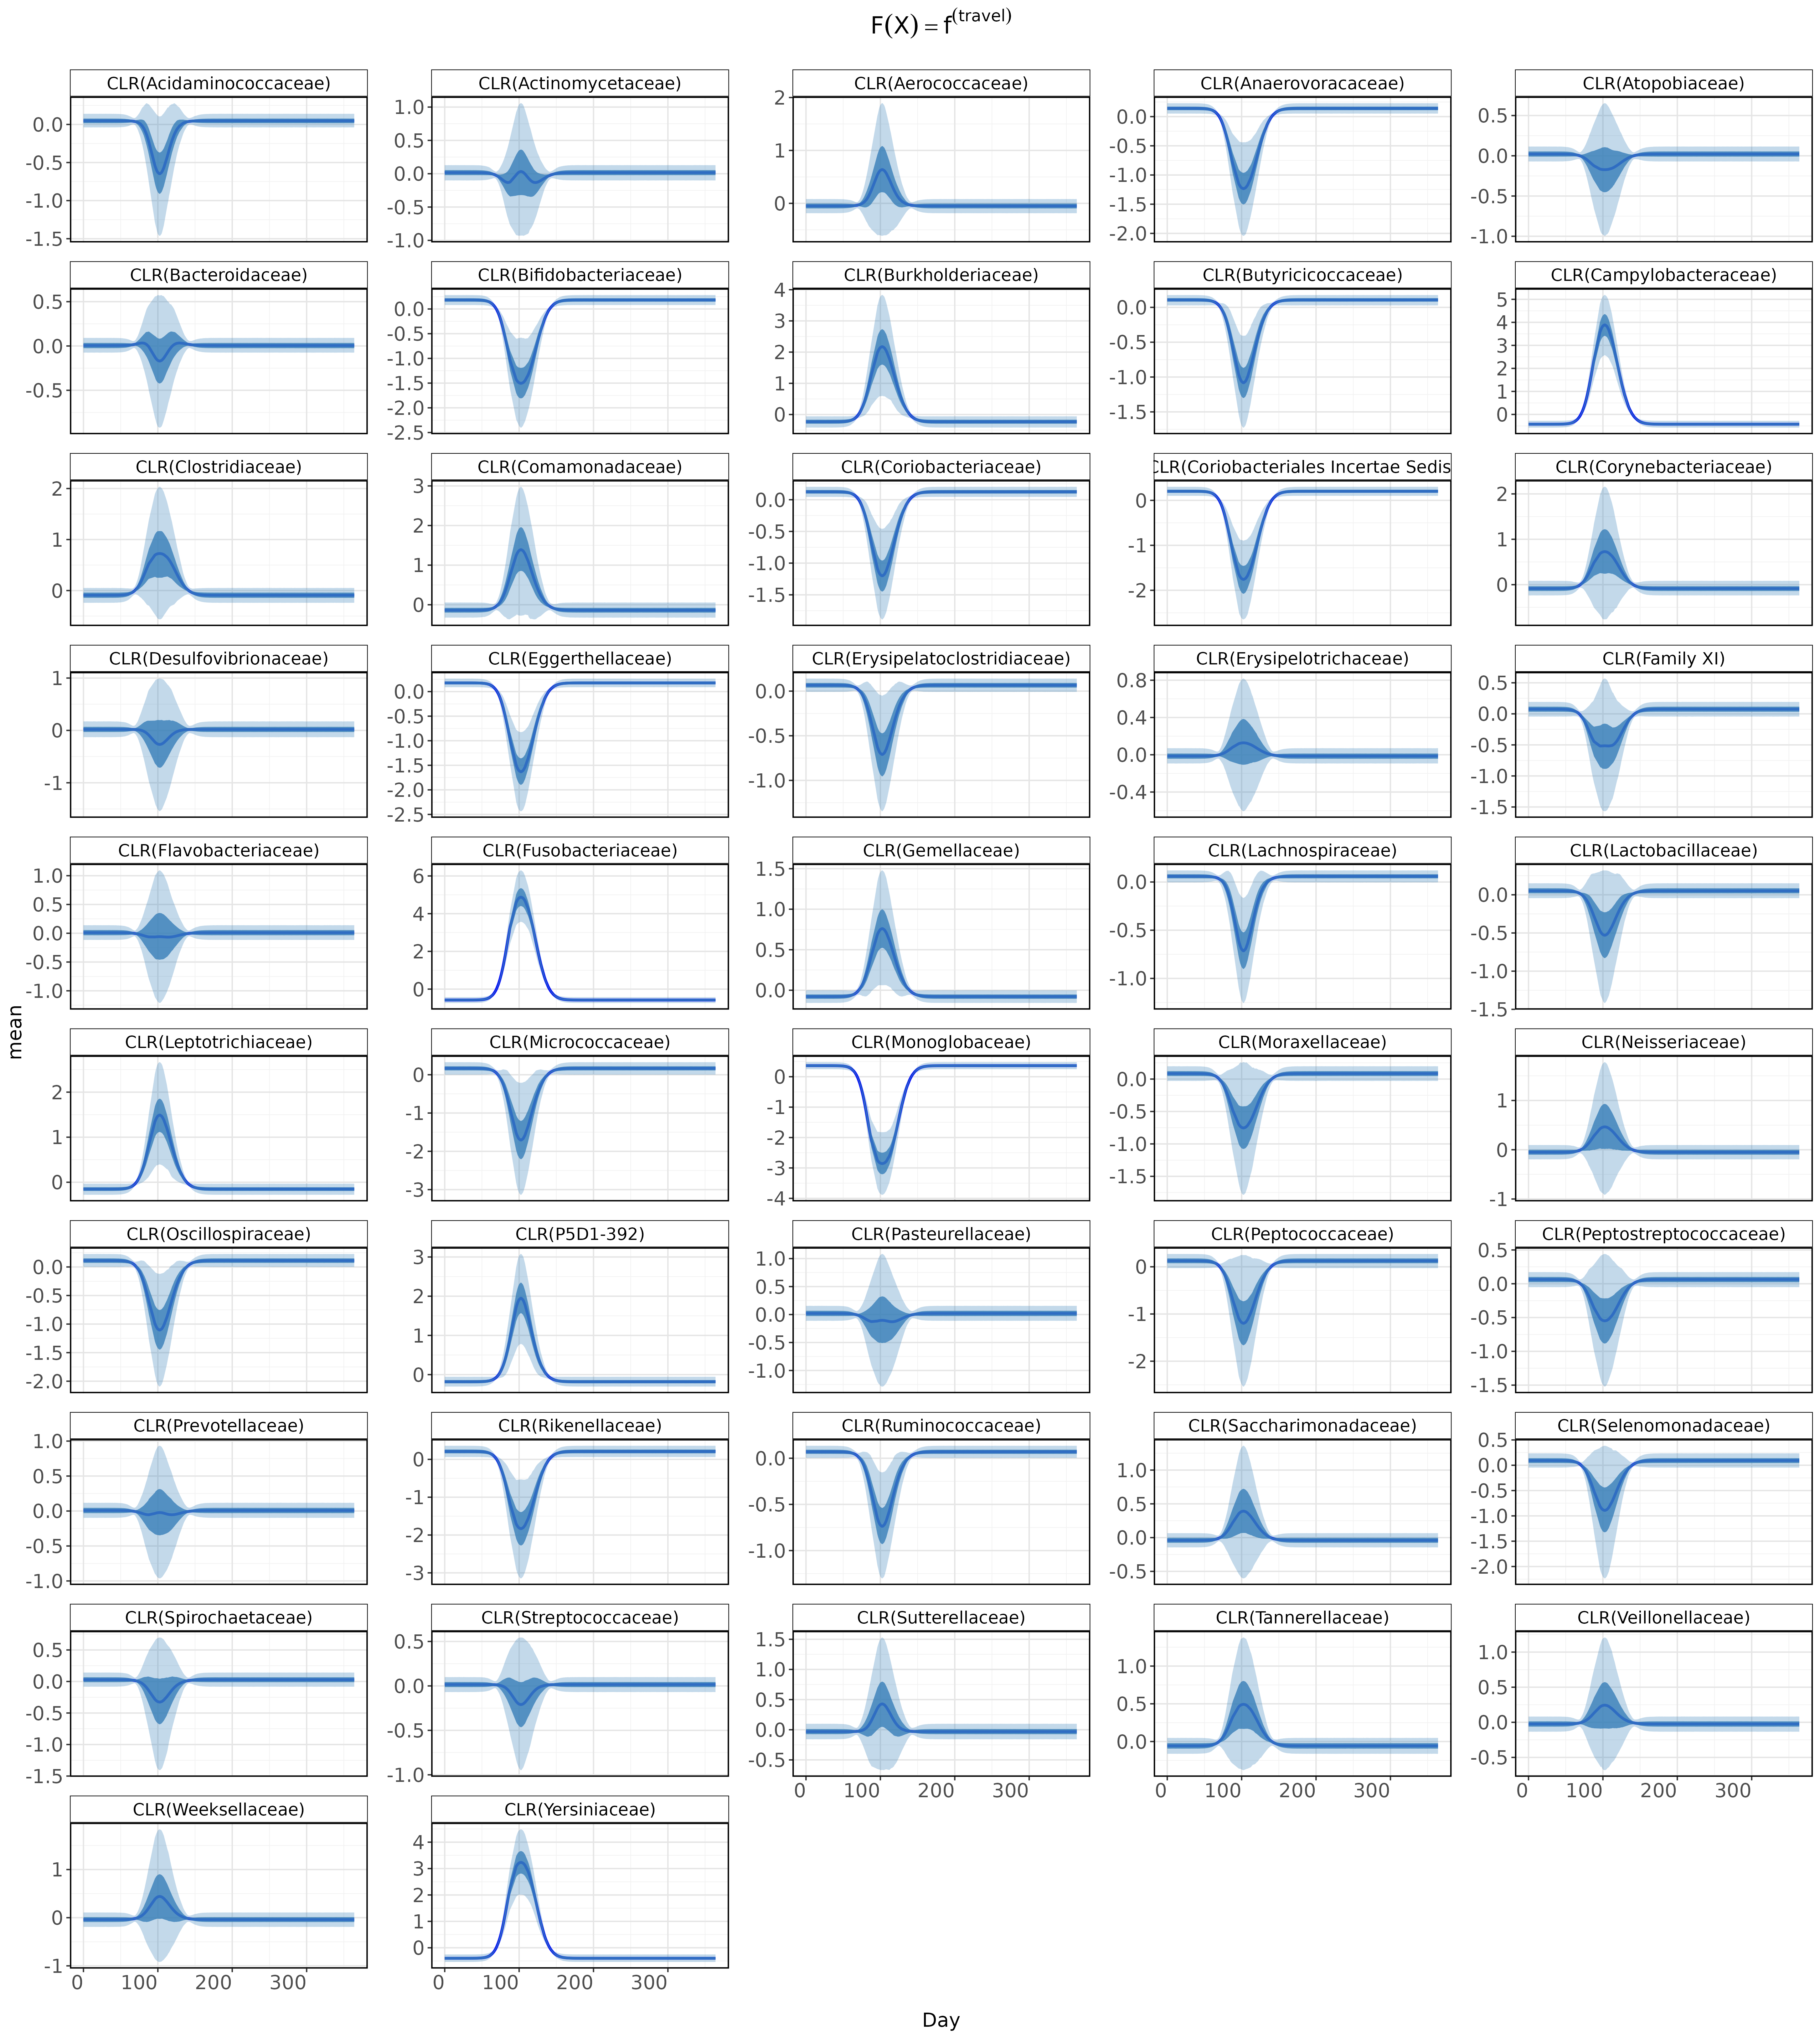}
    \caption{MultiAddGPs Posterior for the travel intervention effect $\mathbf{f}^{\text{(travel)}}$ in the Longitudinal Microbiome Study}
    \label{fig:Long_travel}
\end{figure}

\bibliography{bibliography}       % Bibliography file (usually '*.bib')

\end{document}
